# Supplementary material for: Document Haystacks: Vision-Language Reasoning Over Piles of 1000+ Documents
Source: arXiv:2411.16740 source file (2024-12-06)
Supplement: Supplementary file 1 [file X_suppl.tex]

\clearpage
\maketitlesupplementary

\section{Evaluation}
\begin{figure}[t]
    \begin{tcolorbox}[colframe=black, colback=white, coltitle=black, title=\centering\textbf{Evaluation Prompt}, sharp corners=southwest, enhanced, fonttitle=\bfseries, coltitle=white, colbacktitle=black, boxrule=0.8mm, arc=4mm]
        \begin{quote}
            \textbf{Task:} You are an evaluator. Compare the Predicted Answer with the True Answer and determine if the Predicted Answer is Correct or Incorrect.\\
            \textbf{Instructions:}
            \begin{itemize}[label=-]
                \item If the Predicted Answer provides the same information or a reasonable interpretation of the True Answer, respond with \texttt{Correct.}
                \item If the Predicted Answer does not match or does not reasonably interpret the True Answer, respond with \texttt{Incorrect.}
            \end{itemize}
            \textbf{Important:} Answer only with \texttt{Correct} or \texttt{Incorrect}—no explanations.\\
            \textbf{Input:}
            \begin{itemize}[label=-]
                \item \textbf{Question:} \{ \}
                \item \textbf{True Answer:} \{ \}
                \item \textbf{Predicted Answer:} \{ \}
            \end{itemize}
        \end{quote}
    \end{tcolorbox}
    \captionof{figure}{\textbf{The Designed Prompt for GPT Evaluation.}}
    \label{supp:eval_prompt}
\end{figure}

\textbf{GPT-based evaluation vs. traditional evaluation.} In the open visual question answering (VQA) task, the model can generate the answer in diverse format and it is hard to accurately evaluate the generated answer. 

Traditional evaluation metric such as,  \textit{Exact Match},  measures the percentage of questions where the predicted answer exactly matches one of the target answers, giving a score of zero even when the prediction is only slightly different from the correct answer.
The issue with this evaluation is that language is inherently flexible, and there can be various texts to express the same idea (\eg, ``the dog is sleeping'' vs. ``a sleeping dog'').
This flexibility often results in the \textit{Exact Match} metric failing to capture the true capability of the model sometimes. 
As shown in Fig.~\ref{supp:eval_metric1}, we show examples of zero-shot predictions from Qwen2-VL, generated without any specialized prompt design. It is clear that the \textit{Exact Match} metric fails to evaluate the accuracy of responses in this setting.
To address this, we seek a more reasonable evaluation metric that accounts for this linguistic flexibility.
With the recent advancements in LLMs, GPT-based evaluations are growing in popularity. due to their closer alignment with human behavior in interpreting language.
We carefully design an evaluation prompt for GPT to score the predicted answer against the true answer. The evaluation prompt is structured in Fig~\ref{supp:eval_prompt}.

\begin{figure}[t]
	\begin{center}
        \includegraphics[width=1.0\linewidth]{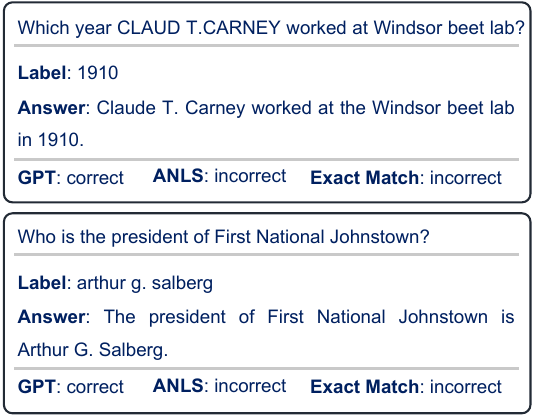}
	\end{center}
	\captionsetup{font=small}
        \vspace{-3mm}
        \caption{\textbf{Zero-Shot VQA without using Task-Specific Prompt.} Without limiting the output space, traditional metrics cannot evaluate model performance even when the model's answer is correct.}
	\label{supp:eval_metric1}
\end{figure}

\begin{figure}[t]
	\begin{center}
        \includegraphics[width=1.0\linewidth]{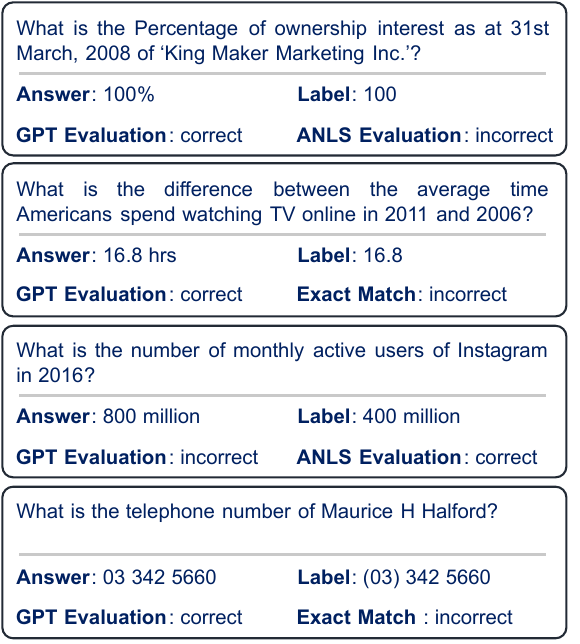}
	\end{center}
	\captionsetup{font=small}
        \vspace{-3mm}
        \caption{\textbf{Zero-Shot VQA with using Task-Specific Prompt.} Even when the output space is limited, traditional metrics sometimes fail to evaluate model performance correctly, even if the model's answer is correct.}
	\label{supp:eval_metric2}
\end{figure}

We validate the consistency of the proposed GPT-based evaluation with human judgments, aiming to demonstrate its effectiveness compared to traditional metrics, \ie, \textit{Exact Match} and \textit{ANLS}. Note that for \textit{ANLS}, we consider a similarity score greater than 0.8 as correct.
As illustrated in Fig.~~\ref{supp:eval_metric2}, traditional metrics can sometimes misjudge zero-shot prediction. This limitation becomes evident in scenarios where the flexibility of responses is crucial.
%
% While task-specific prompts can guide models to provide more constrained outputs, they are often impractical in real-world applications as it is difficult for us to know the distribution of answers beforehand.
%∂
Note that we explicitly ask the model to ``Answer the question using a single word or phrase.''~\footnote{\url{https://github.com/EvolvingLMMs-Lab/lmms-eval}} This prompt ensures brevity and facilitates a fair comparison between predicted and target answers. 

We report the performance of different evaluation metrics on DocHaystack-100 and InforHaystack-100 in Tab.~\ref{tab:eval_metrics}. The results show that the introduced GPT-based metric aligns closely with human evaluation, outperforming traditional metrics.
Based on these experimental results, we choose GPT-based evaluation for better accuracy.

\begin{table}[h]
\centering
\resizebox{1.0 \linewidth}{!}{
    \begin{tabular}{c ccc}
    \toprule
    Evaluation Metric& DocHaystack 100& InfoHaystack 100\\
    % \midrule
    \cmidrule(r){1-1} \cmidrule(lr){2-2} \cmidrule(lr){3-3}
    Human & 78.90 & 62.58 \\
    Exact Match & 69.72 & 58.71 \\
    ANLS & 73.39 & 60.65 \\
    \rowcolor{TealBlue}
    GPT & 78.90 & 62.58 \\
    \bottomrule
    \end{tabular}
}
\caption{\textbf{Accuracy of Qwen2-VL on DocHaystack-100 and InfoHaystack-100.} We report different accuracy using different evaluation metrics.}
\label{tab:eval_metrics}
\end{table}

\section{Image Retrieval}

We select retrieved images based on their similarity to the question and present the three most relevant images retrieved using different methods (\ie, V-RAG-based retrieval, CLIP-based retrieval, SigLIP-based retrieval, OpenCLIP-based Retrieval): Fig.~\ref{supp:retrieval1}~--~\ref{supp:retrieval3} for DocHaystack and Fig.~\ref{supp:retrieval4}~--~\ref{supp:retrieval6} for InfoHaystack.
In these figures, the red box outside the retrieved image highlights the ground truth image paired with the question. The red box within each retrieved image shows the related information to the question. The yellow box in the ground truth image paired with the question shows the ground truth answer for the question. As can be seen in these figures, our proposed V-RAG performs well in question-related image retrieval.

\begin{figure*}[t!]
	\begin{center}
        \includegraphics[width=\linewidth]{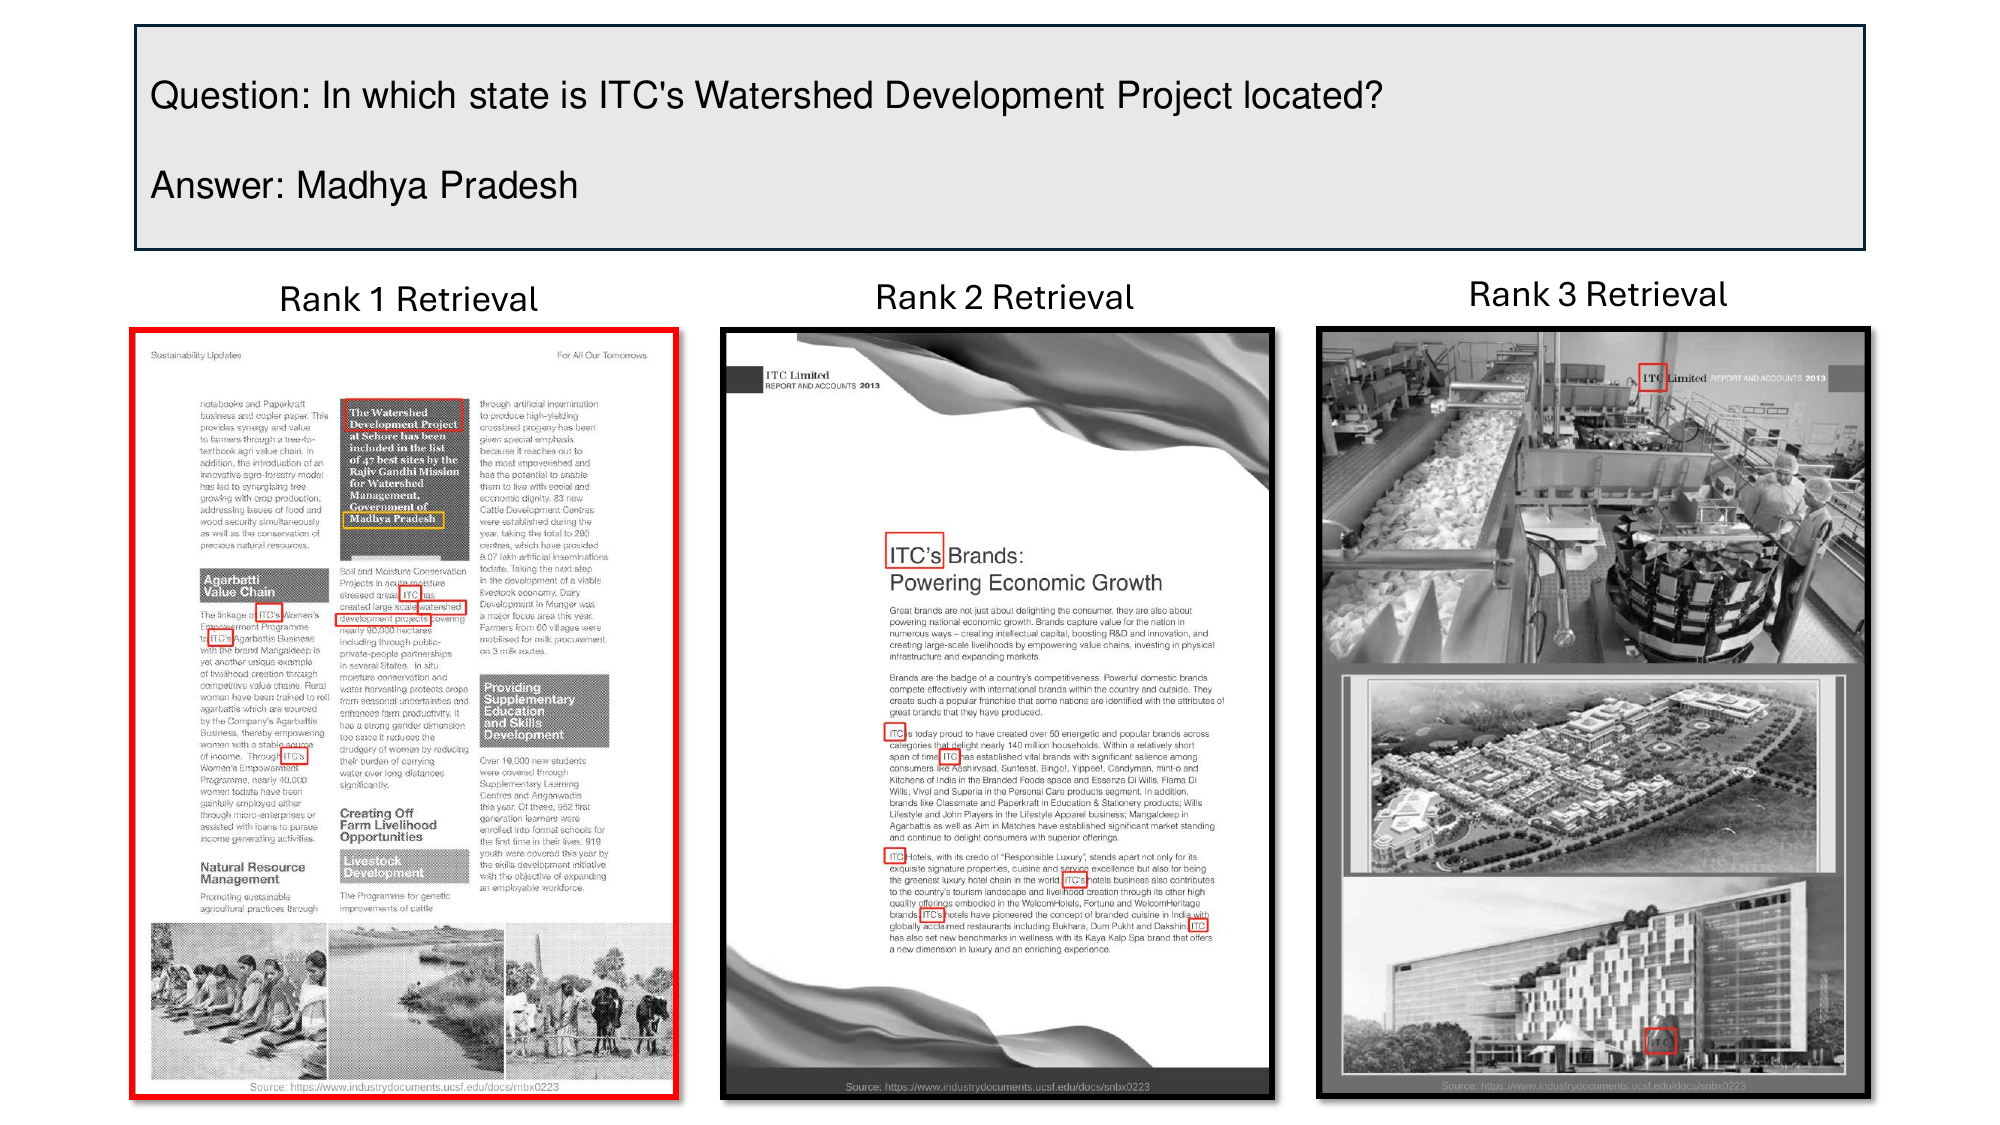}
	\end{center}
	\captionsetup{font=small}
	\caption{The three images most similar to the question retrieved using V-RAG in DocHaystack. The red box highlights the ground truth image paired with the question.
    % The red circle in each image shows the related information to the question. The yellow circle in the ground truth image paired with the question shows the ground twruth answer for the question.
    }
	\label{supp:retrieval1}
    \vspace{-0.3cm}
\end{figure*}

\begin{figure*}[t!]
	\begin{center}
        \includegraphics[width=\linewidth]{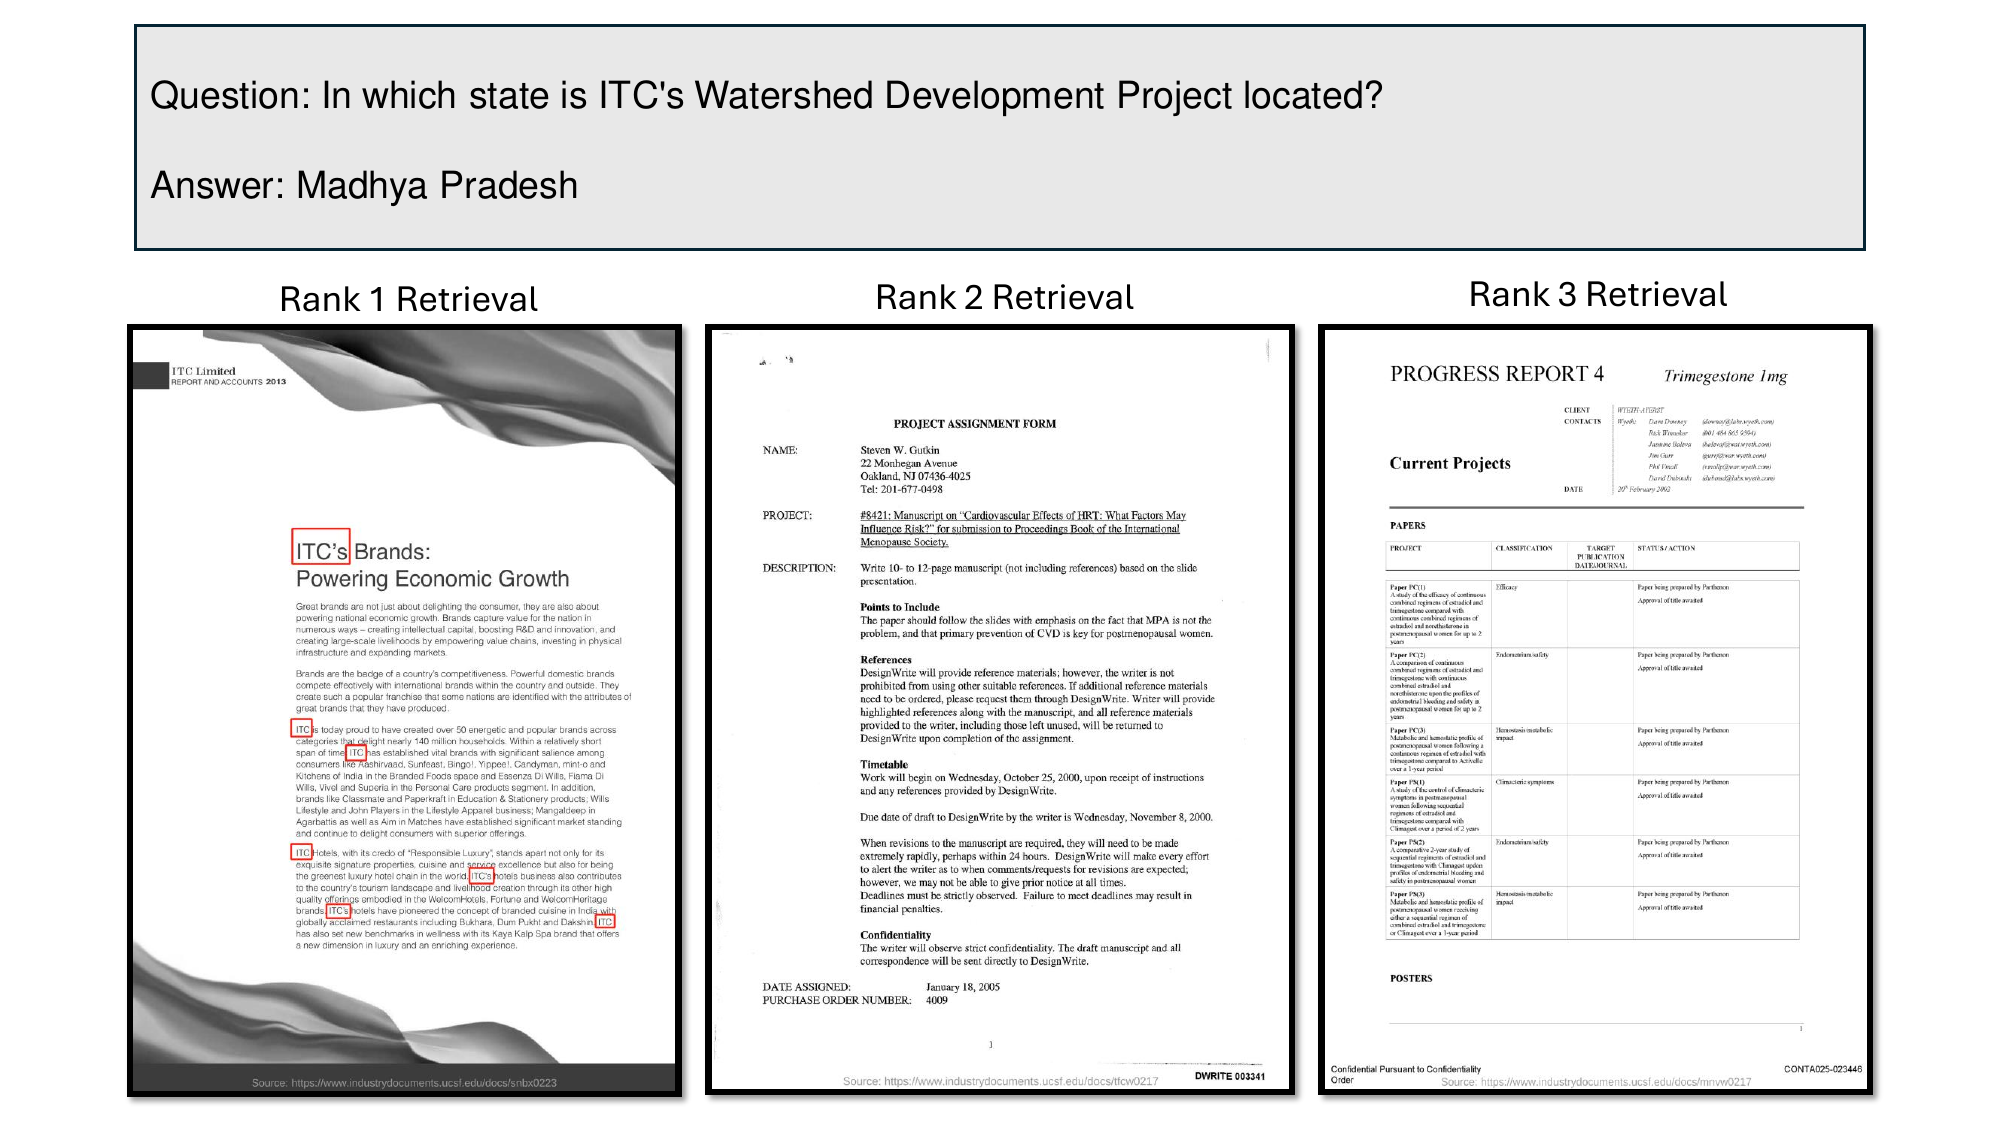}
	\end{center}
	\captionsetup{font=small}
	\caption{The three images most similar to the question retrieved using CLIP in DocHaystack. The red box highlights the ground truth image paired with the question.
    % The red circle in each image shows the related information to the question. The yellow circle in the ground truth image paired with the question shows the ground truth answer for the question.
    }
	\label{supp:retrieval2}
    \vspace{-0.3cm}
\end{figure*}

\begin{figure*}[t!]
	\begin{center}
        \includegraphics[width=\linewidth]{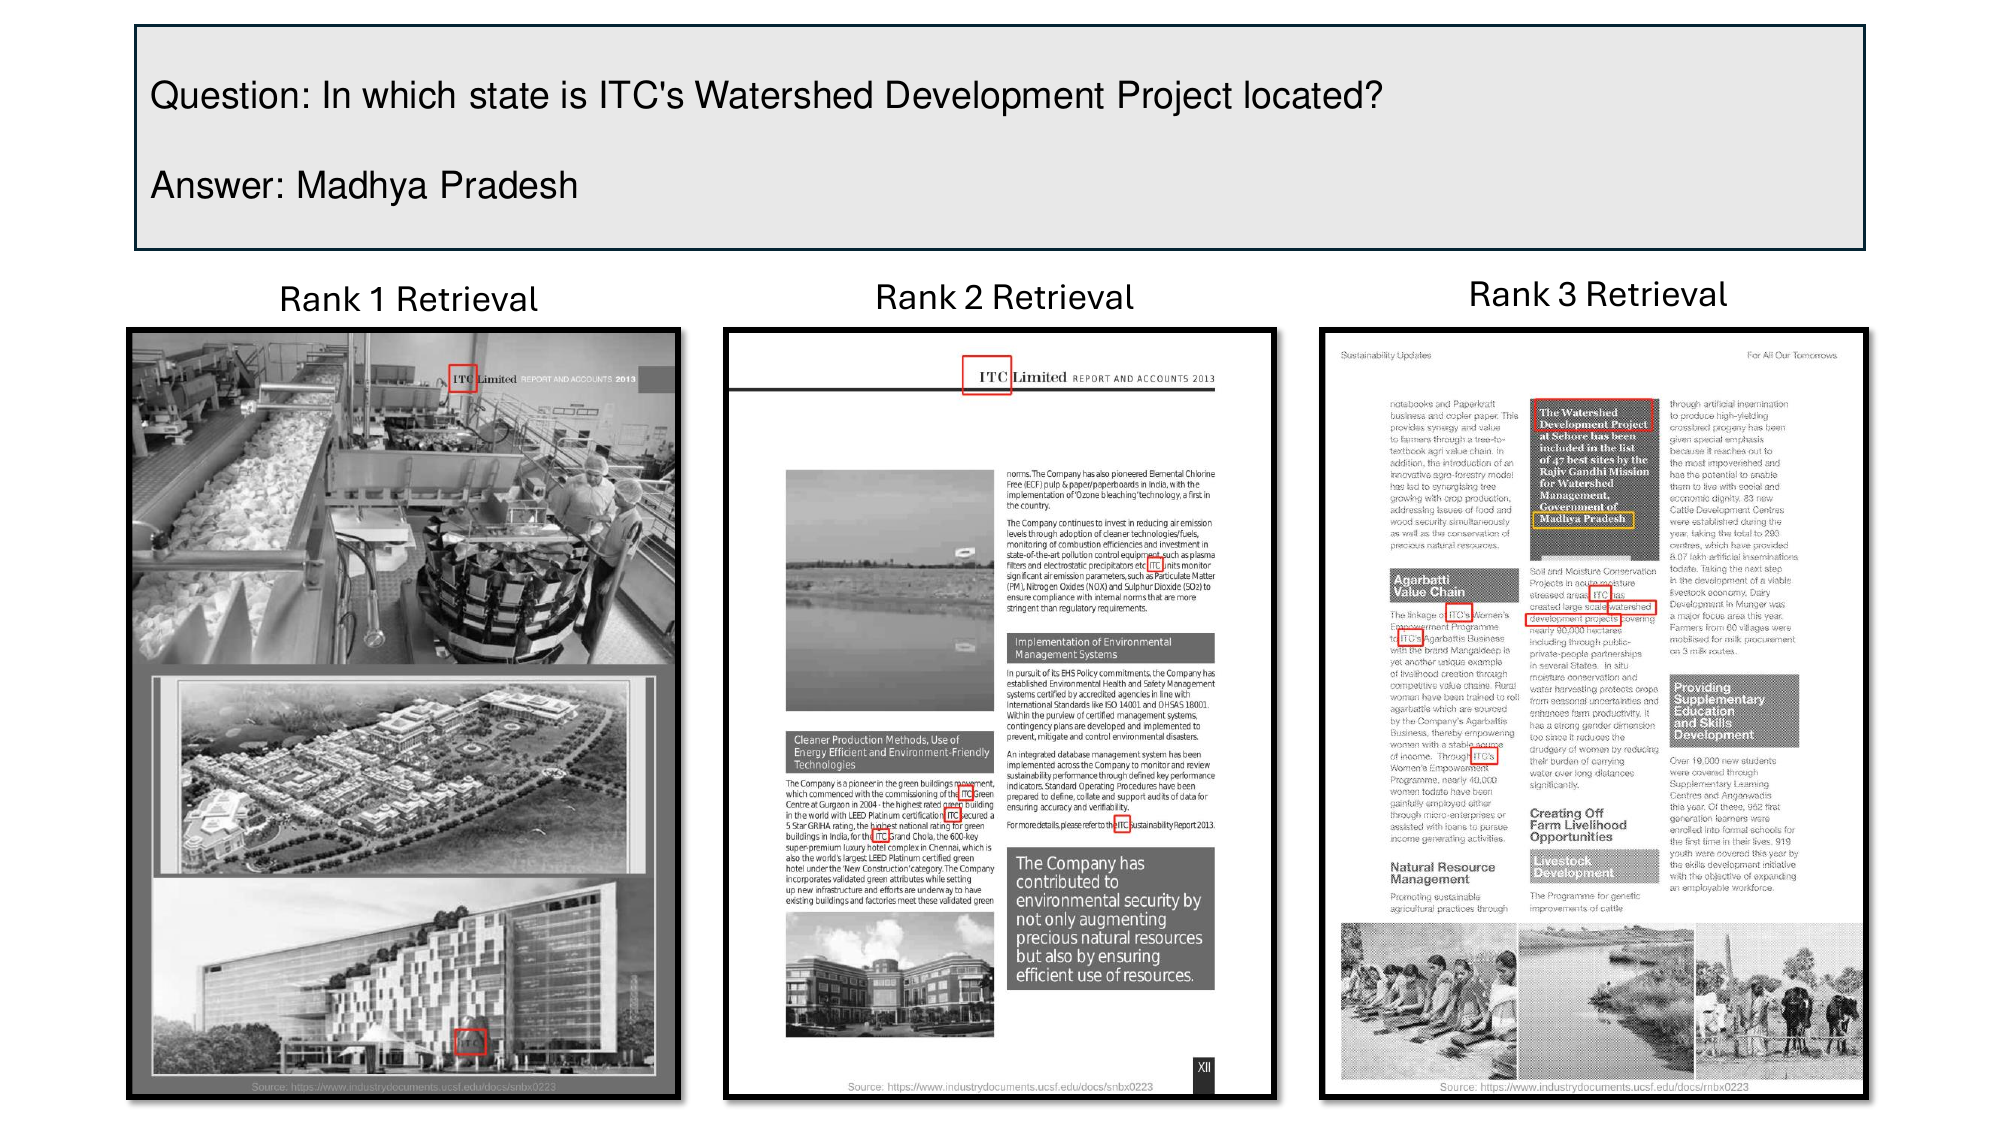}
	\end{center}
	\captionsetup{font=small}
	\caption{The three images most similar to the question retrieved using SigLIP in DocHaystack. The red box highlights the ground truth image paired with the question.
    % The red circle in each image shows the related information to the question. The yellow circle in the ground truth image paired with the question shows the ground truth answer for the question.
    }
	\label{supp:retrieval3}
    \vspace{-0.3cm}
\end{figure*}

\begin{figure*}[t!]
	\begin{center}
        \includegraphics[width=\linewidth]{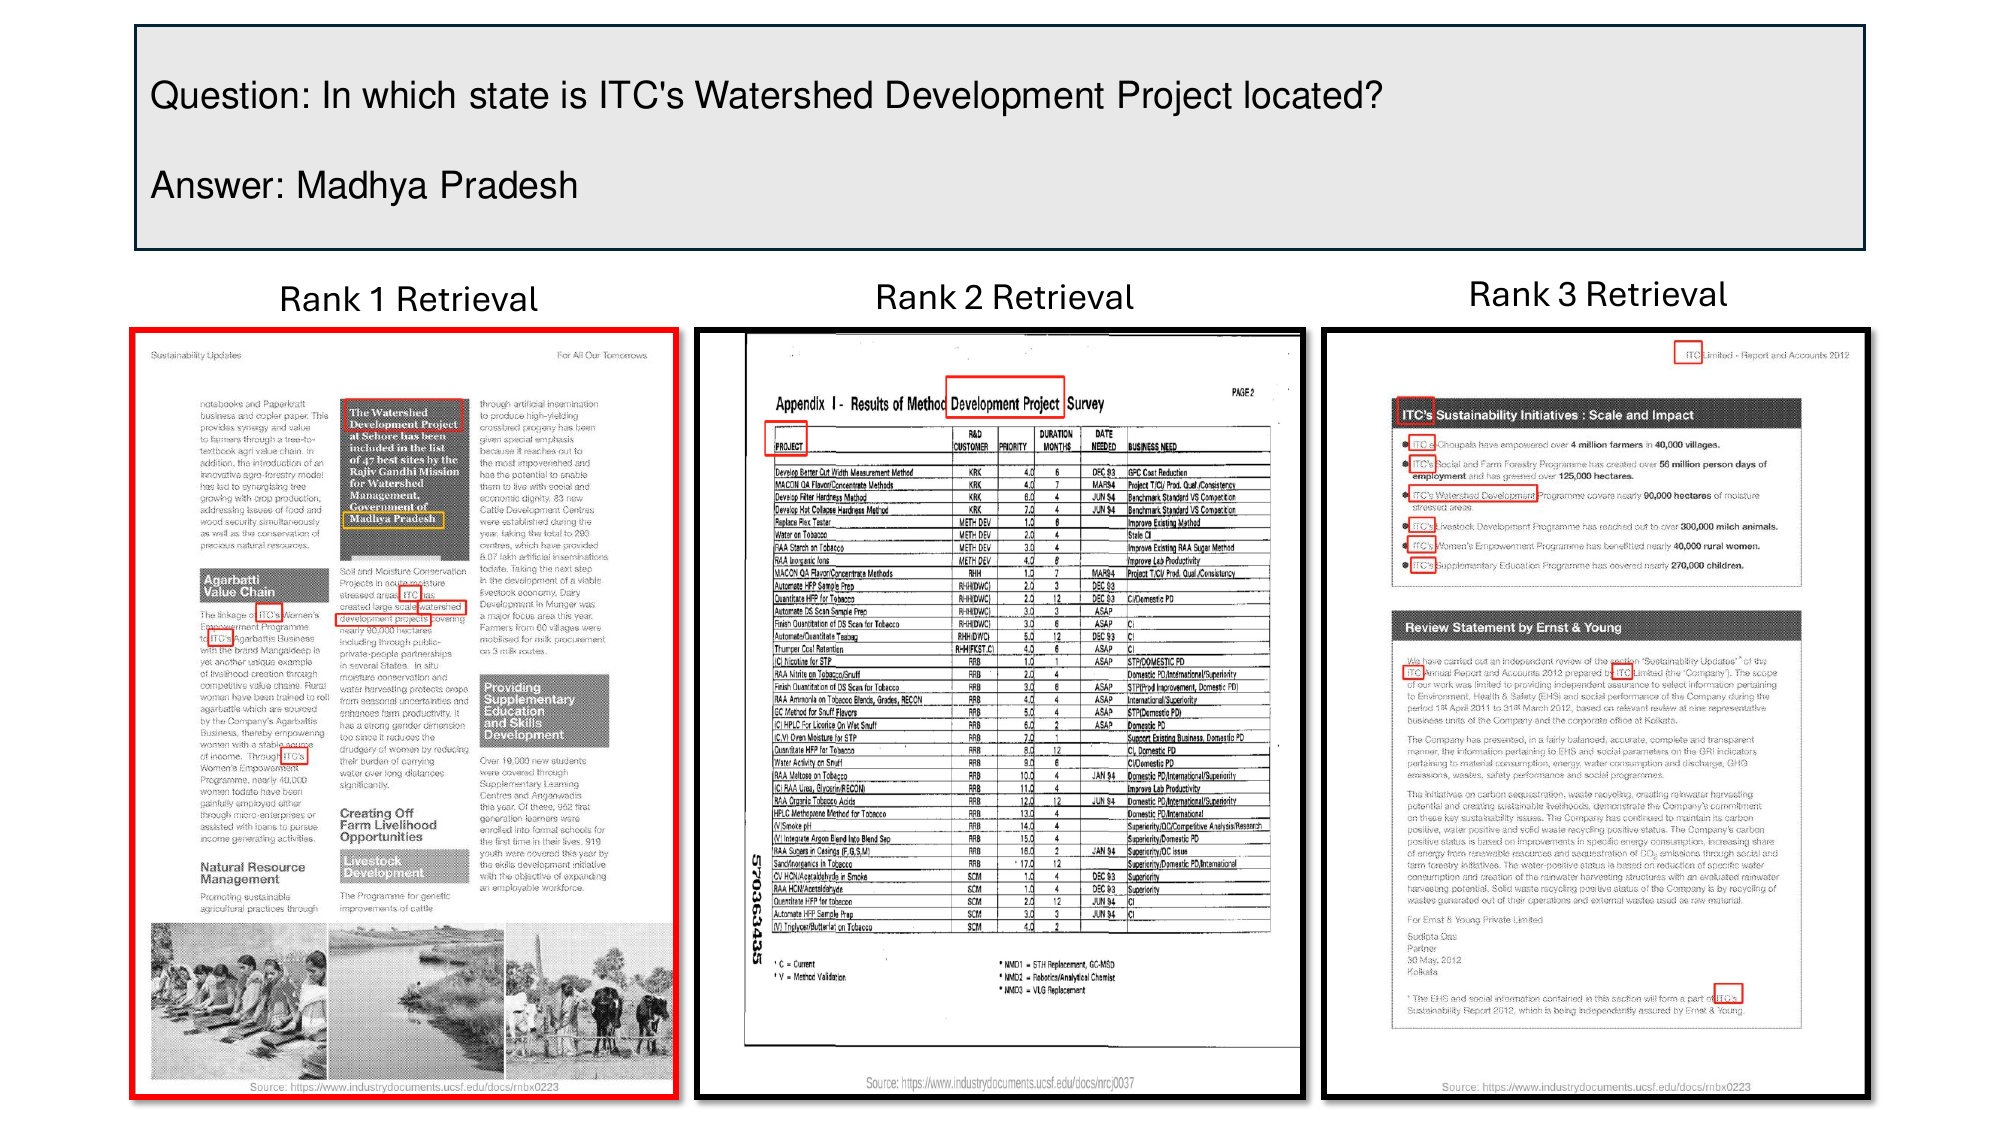}
	\end{center}
	\captionsetup{font=small}
	\caption{The three images most similar to the question retrieved using OpenCLIP in DocHaystack. The red box highlights the ground truth image paired with the question.
    % The red circle in each image shows the related information to the question. The yellow circle in the ground truth image paired with the question shows the ground truth answer for the question.
    }
	\label{supp:retrieval4}
    \vspace{-0.3cm}
\end{figure*}

\begin{figure*}[t!]
	\begin{center}
        \includegraphics[width=\linewidth]{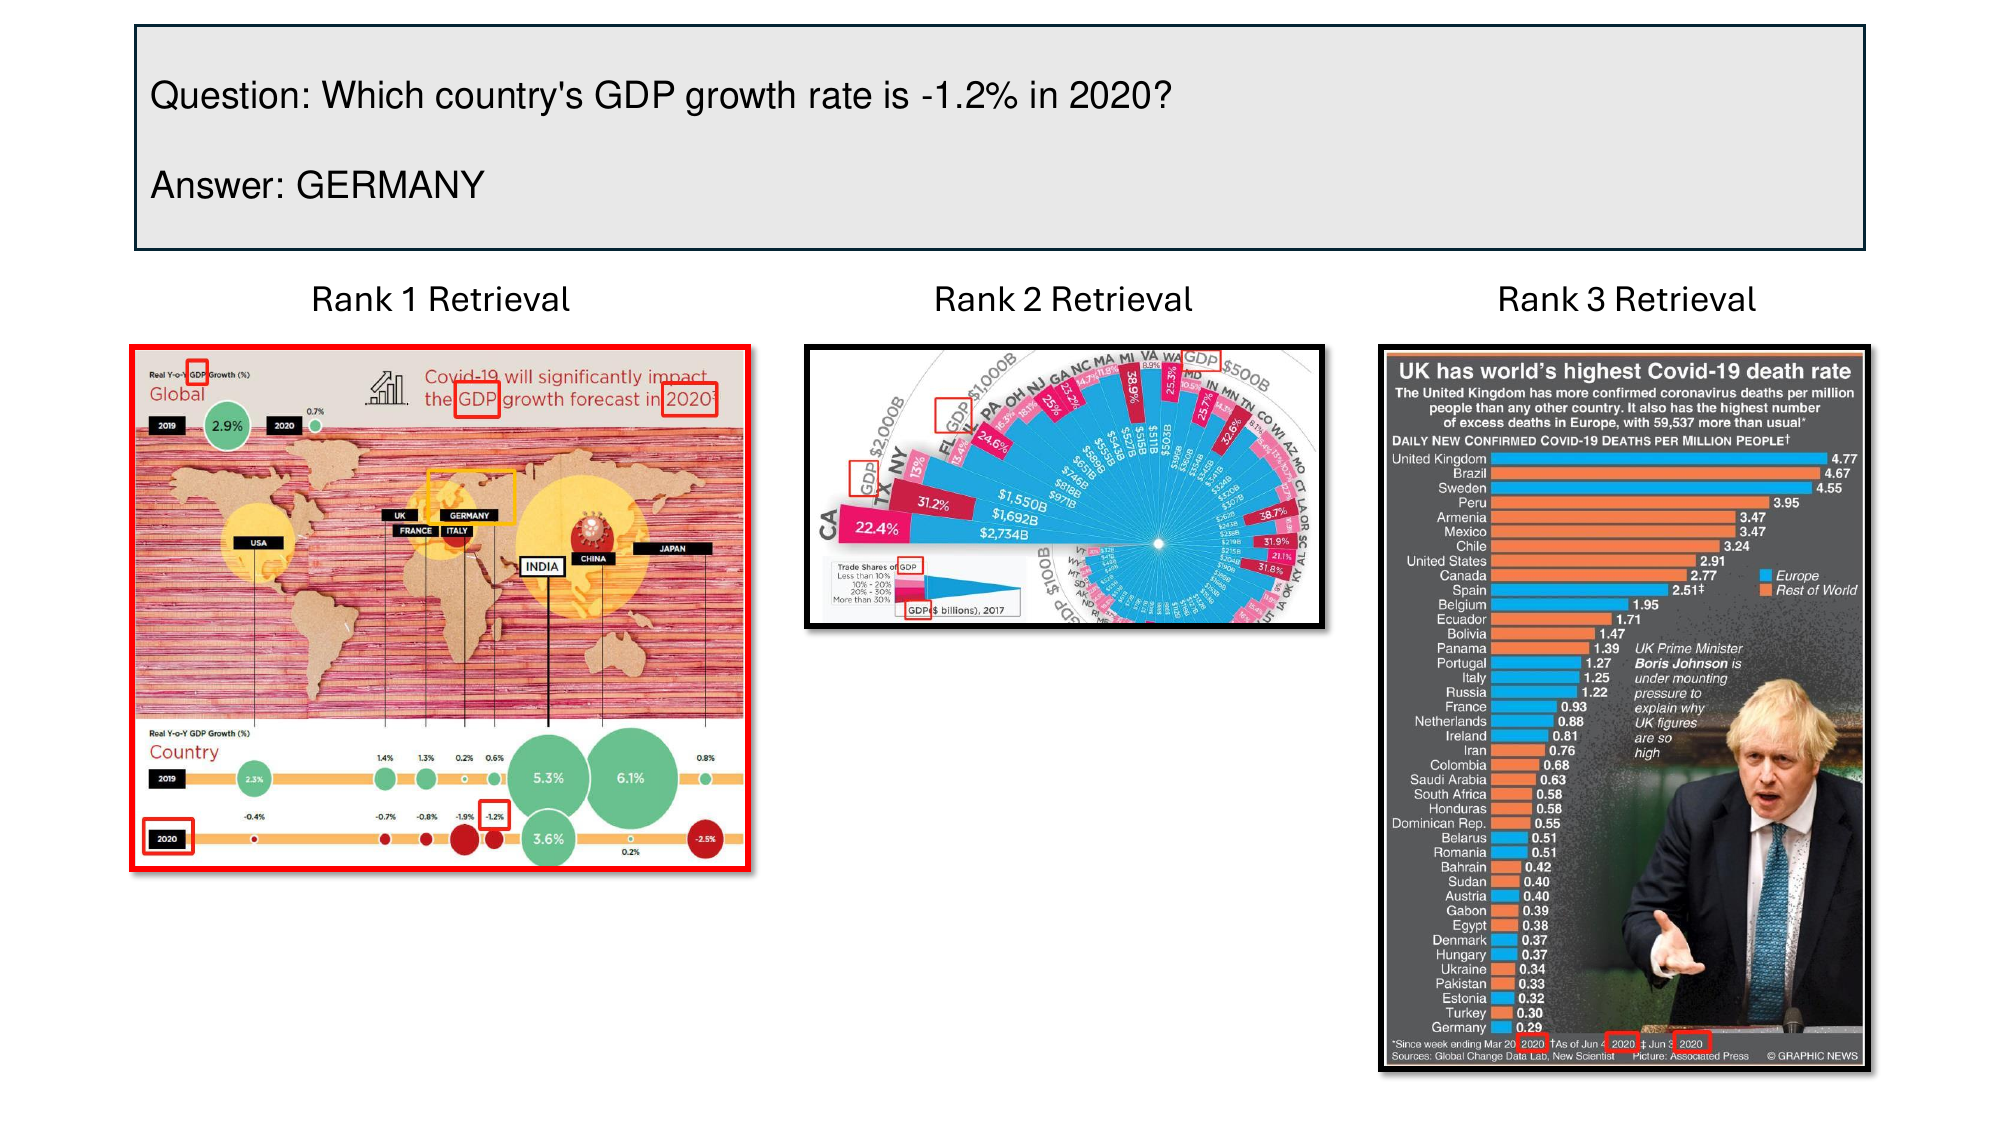}
	\end{center}
	\captionsetup{font=small}
	\caption{The three images most similar to the question retrieved using V-RAG in InfoHaystack. The red box highlights the ground truth image paired with the question.
    % The red circle in each image shows the related information to the question. The yellow circle in the ground truth image paired with the question shows the ground truth answer for the question.
    }
	\label{supp:retrieval5}
    \vspace{-0.3cm}
\end{figure*}

\begin{figure*}[t!]
	\begin{center}
        \includegraphics[width=\linewidth]{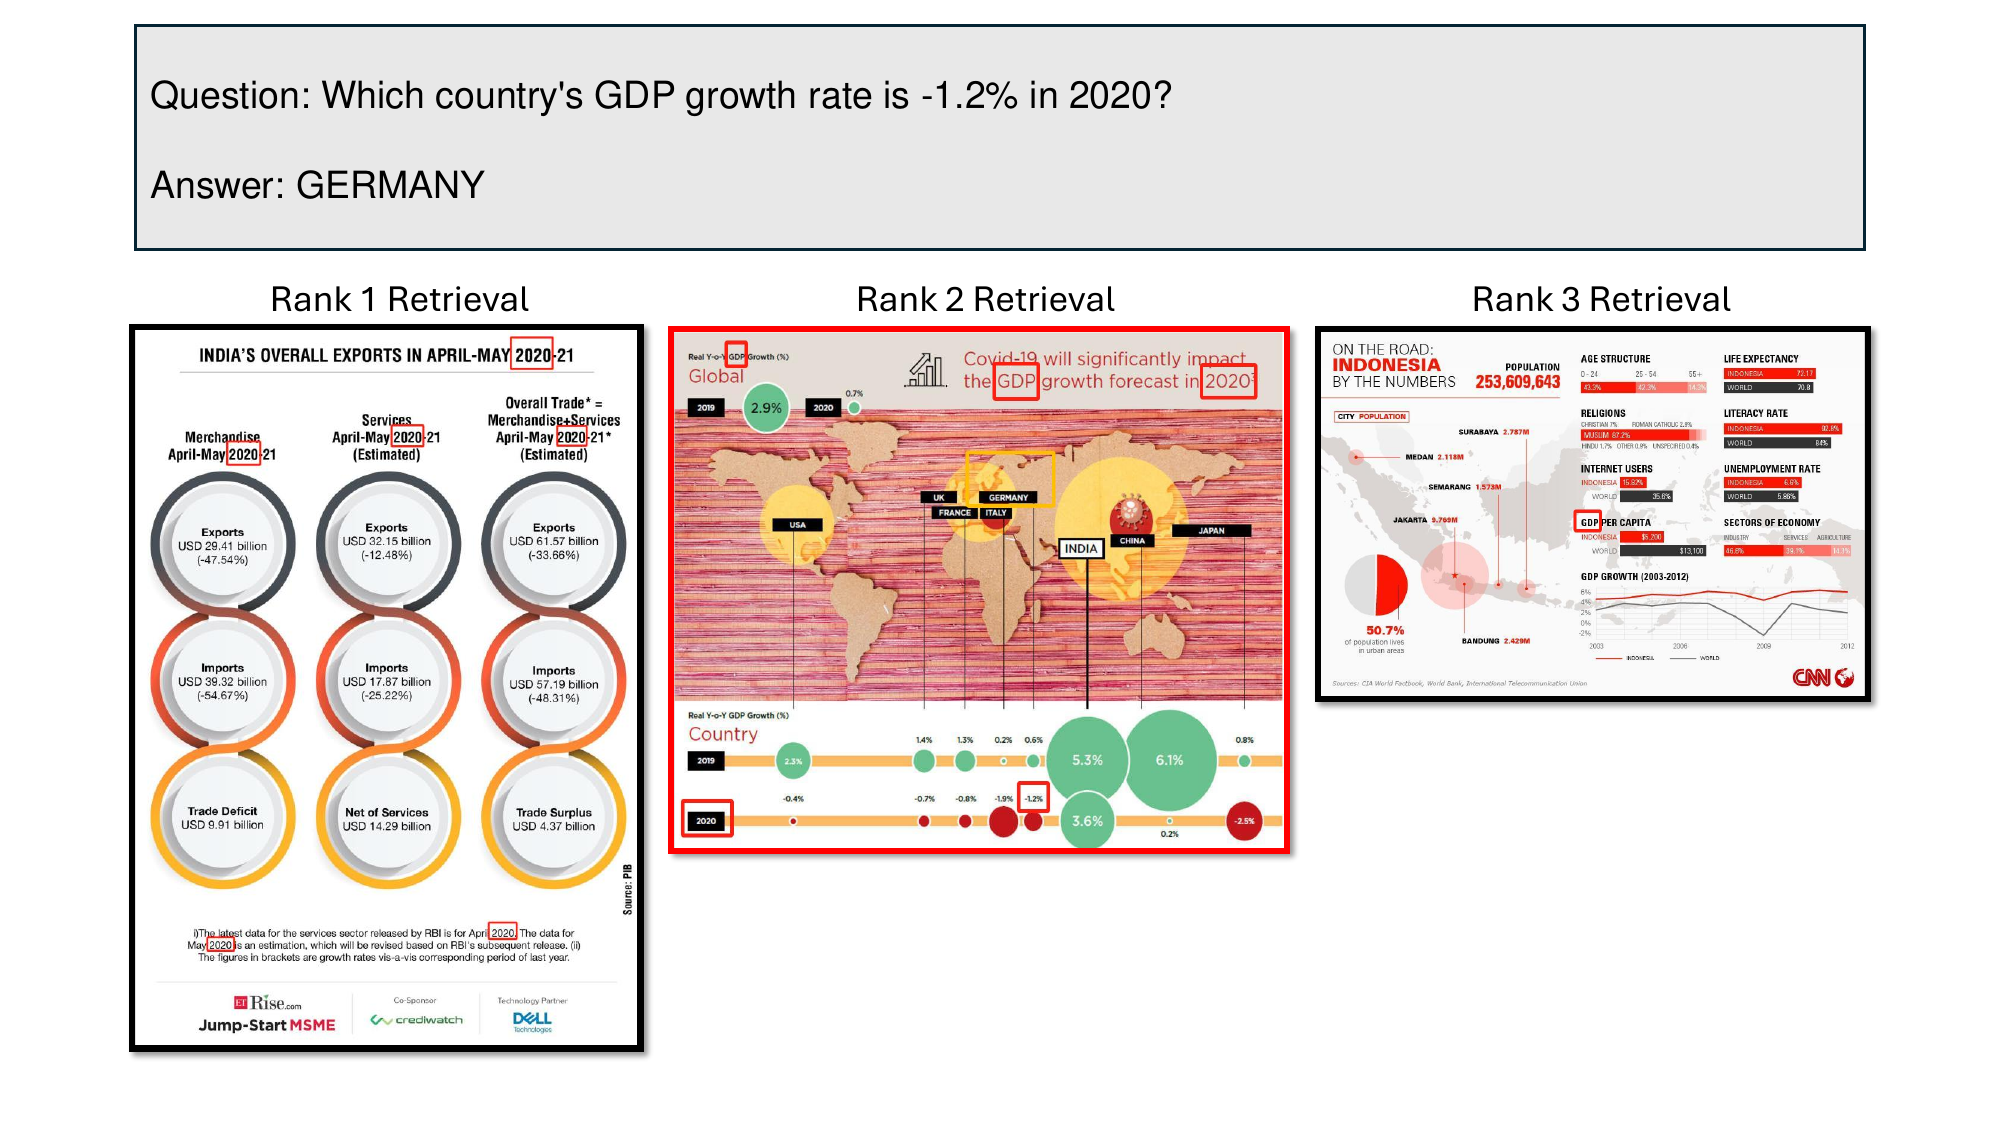}
	\end{center}
	\captionsetup{font=small}
	\caption{The three images most similar to the question retrieved using CLIP in InfoHaystack. The red box highlights the ground truth image paired with the question.
    % The red circle in each image shows the related information to the question. The yellow circle in the ground truth image paired with the question shows the ground truth answer for the question.
    }
	\label{supp:retrieval6}
    \vspace{-0.3cm}
\end{figure*}

\begin{figure*}[t!]
	\begin{center}
        \includegraphics[width=\linewidth]{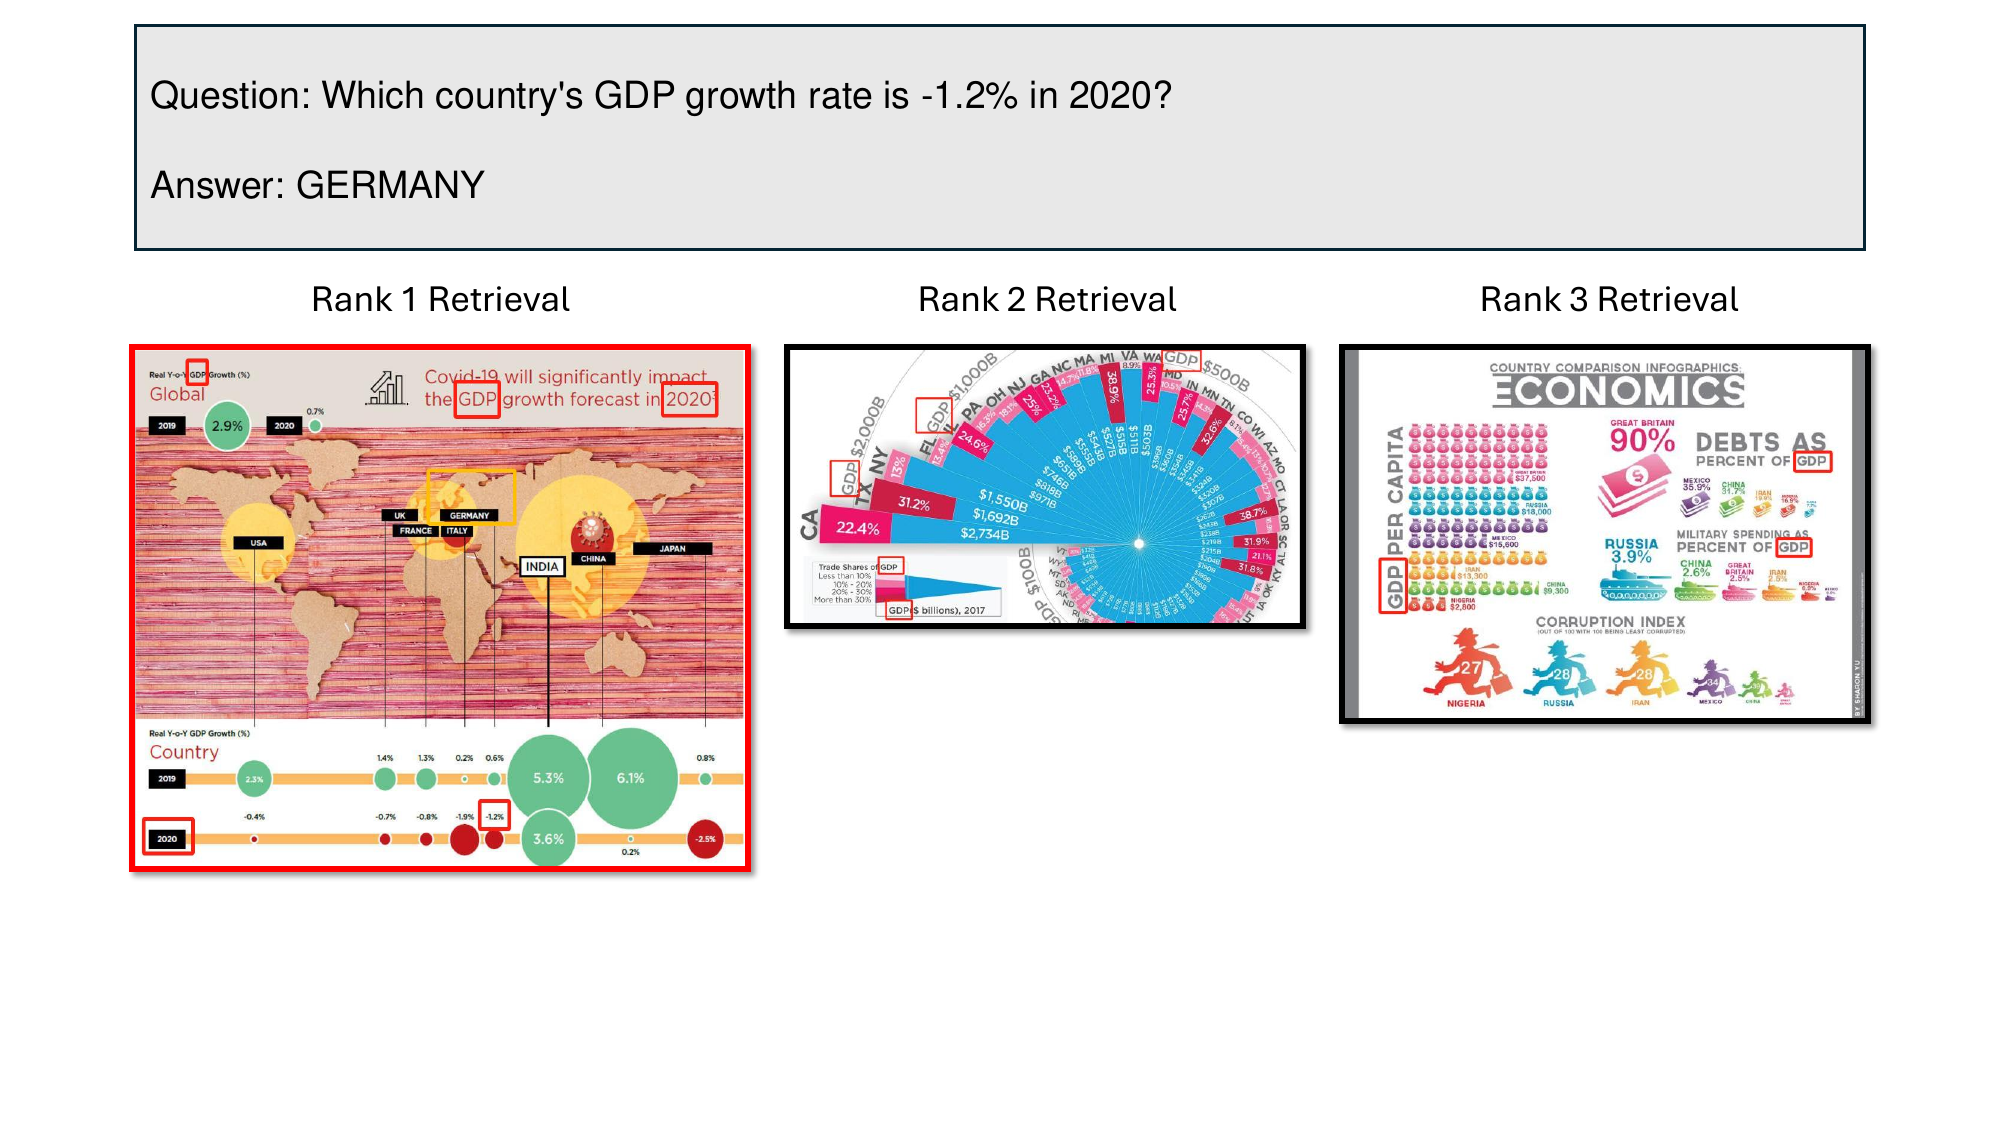}
	\end{center}
	\captionsetup{font=small}
	\caption{The three images most similar to the question retrieved using SigLIP in InfoHaystack. The red box highlights the ground truth image paired with the question.
    % The red circle in each image shows the related information to the question. The yellow circle in the ground truth image paired with the question shows the ground truth answer for the question.
    }
	\label{Rank_SIGLIP_Info}
    \vspace{-0.3cm}
\end{figure*}

\begin{figure*}[t!]
	\begin{center}
        \includegraphics[width=\linewidth]{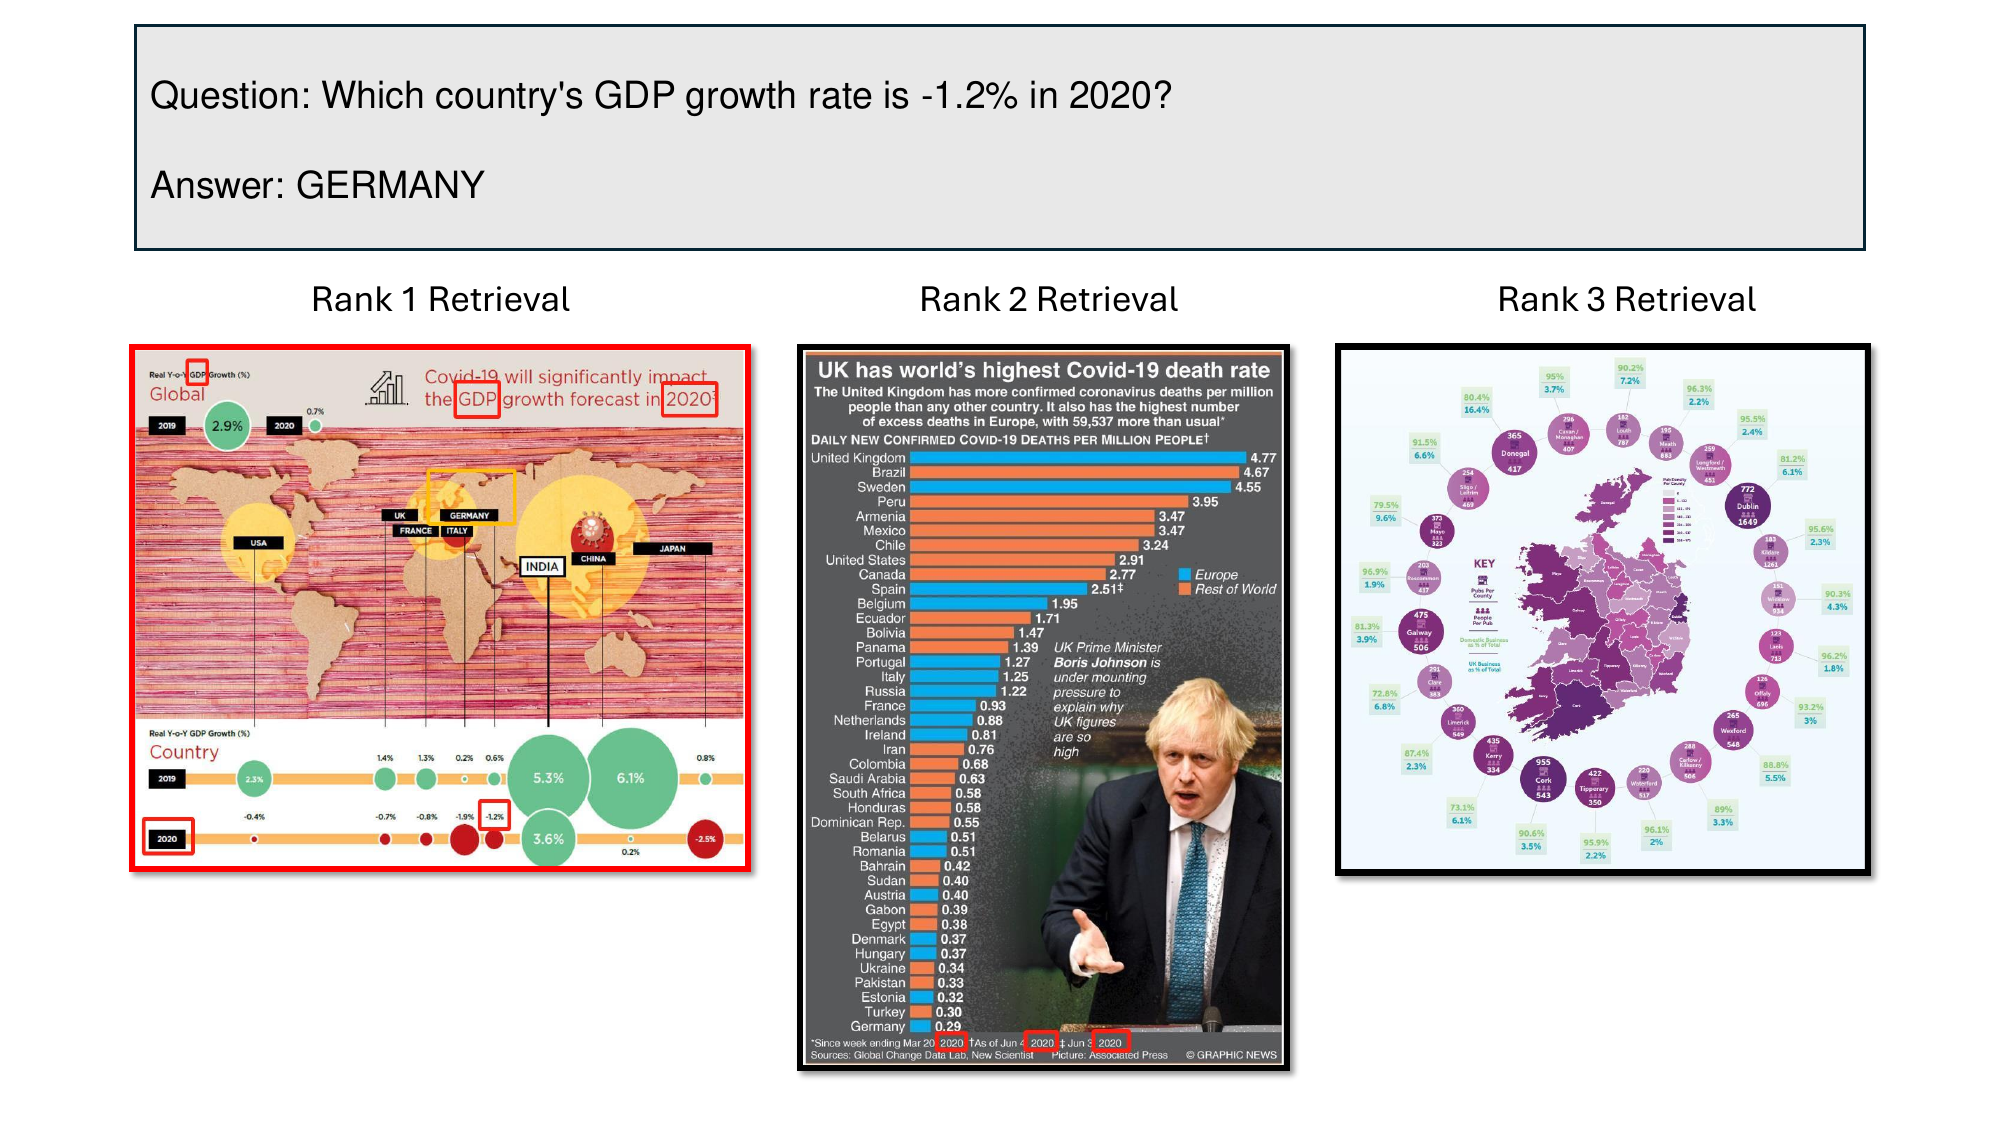}
	\end{center}
	\captionsetup{font=small}
	\caption{The three images most similar to the question retrieved using OpenCLIP in DocHaystack. The red box highlights the ground truth image paired with the question.
    % The red circle in each image shows the related information to the question. The yellow circle in the ground truth image paired with the question shows the ground truth answer for the question.
    }
	\label{Rank_OpenCLIP_Info}
    \vspace{-0.3cm}
\end{figure*}

% \section{General-Question LLM Filtering}
% \subsection{DocHaystack}
\clearpage
% \section{General-Question LLM Filtering}
% \subsection{DocHaystack}

\section{Question Filtering Pipeline}

General questions can typically be answered from multiple documents, with several possible correct answers. For example, the question ``Who wrote the letter'' is a general question that can be answered by any document containing a letter.
Generic Knowledge refers to information or facts that are widely accessible and can be answered using general world knowledge, often independent of specific visual or contextual cues from accompanying content, such as images. For example, the question ``How many events were featured in the 2014 Winter Olympics?'' is a generic knowledge that can be answered without accessing any image.
In visual question answering tasks such as DocVQA and InfographicVQA, generic knowledge introduces a language bias when large language models (LLMs) rely on pre-existing knowledge rather than visual content, thereby undermining the focus on image-based reasoning.
Therefore, it is important to exclude such questions to evaluate the true image-based reasoning capability of models.
In this section, we show how we filter the data to extract the specific question.

\subsection{General Question LLM Filtering}
First, we leverage an LLM to filter out the general questions. This approach allows for the automatic filtering of numerous general questions. We give some filtered general questions by LLM here.

\paragraph{DocHaystack}
\begin{itemize}
    \item What does C stand for?
    \item What is the receiver number?
    \item What is the zip code?
    \item What is plotted along the x axis ?
    \item Who wrote the letter?
    \item What is the Fund No.?
    \item What type of report is this?
    \item Who is the client?
    \item What is the description?
    \item What is the name of the company?
\end{itemize}

\paragraph{InfoHaystack}
\begin{itemize}
    \item Who is the player in this picture?
    \item How many salary caps are mentioned?
    \item What percentage are not children?
    \item What percentage are not Americans?
    \item How many resources are listed?
    \item How many employers were surveyed?
    \item How countres are listed here in total?
    \item In which school did he study?
    \item What is the second last solution given?
    \item What is written in the yellow circle?
\end{itemize}

\subsection{General-question manual review}

However, the LLM-based filtering is not entirely accurate. Therefore, in the second stage, we involve manual filtering, where annotators are tasked with filtering out any general questions that were missed by the LLM. The filtered general question by human are as follow.

\paragraph{DocHaystack}
\begin{itemize}
    \item What time is the ‘coffee break’?
    \item What is the year of publication?
    \item What is the name of the person on the from?
    \item Which is the root node in the chart?
    \item What is the no of cut tobacco?
    \item What is the name in the letter head?
    \item What is the exit date from china?
    \item What is the first person name marked in CC?
    \item What is the progress Report number?
    \item In which country is the company located?
\end{itemize}

\paragraph{InfoHaystack}
\begin{itemize}
    \item Where is open carry not permitted?
    \item How many points should protection services include?
    \item How many sharing tools mentioned in this infographic?
    \item What percentage of the survey participants are female?
    \item How many products are associated with blue color?
    \item What is the color mode used for the Web?
    \item Who are the swimming players in the list?
    \item Who made this infographic?
    \item How many symptoms are shown?
    \item Who is represented by green colour?
\end{itemize}

\subsection{Generic knowledge filtering}

After filtering out the general questions, we leverage GPT to filter out the remaining questions that can be answered by generic knowledge. The following is a list of some filtered questions.

\paragraph{DocHaystack}
\begin{itemize}
    \item What is the PO box no. of Biomet Orthopedics, Inc.?
    \item What is the Fax number of ‘Brookstown Inn’?
    \item What is the location for Endocrine society-ENDO 2004 meeting?
    \item Which ‘meeting ‘ was held at New Orleans, LA in January 2004?
    \item For which groups, WEFA, Inc. conducted study in April 1998?
    \item When was Argonne National Laboratory study for Department of Energy conducted?
    \item Where was the NAMS(North American Menopause Society)'s 14th Annual Meeting?
    \item What is ITC's brand of Agarbatti?
    \item Which ‘meeting ‘ was held at Miami Beach, FL in May 2003?
    \item What is the brand name of ITC's snack food?
\end{itemize}

\paragraph{InfoHaystack}
\begin{itemize}
    \item What percent of world's adults have a bank account in the year 2014?
    \item What was India's score in the 2011 cricket world cup final?
    \item What percentage of Apple's revenue comes from iPhone in 2016?
    \item How many teams participated in the 2011 ICC Cricket World Cup?
    \item How many events were featured in the 2014 Winter Olympics?
    \item Which state is the second-largest producer of the Christmas tree in the U.S. in 2008?
    \item How many atomic bomb attacks were made by the U.S. in Japan in 1945?
    \item How many times did Hilary Mantel win the Booker prize?
    \item When was the 2011 cricket world cup final?
    \item What was Microsoft's net income in 2018?
\end{itemize}

\subsection{DocHaystack Final 20 Random Questions}

We randomly sample 20 questions in our final list of DocHaystack as below.

\begin{itemize}
    \item Which was CLAUD T.CARNEY’s high school?
    \item Which ITC Brand has 'Liquid Crystal Freezing Technology'?
    \item When was the study of Charles River Associates done?
    \item In which office does Michael Shapiro work?
    \item In which state is ITC's Watershed Development Project located?
    \item Who is ‘presiding’ TRRF GENERAL SESSION (PART 1)?
    \item How many nomination committee meetings has S. Banerjee attended?
    \item What is the number of Investor Services Committee meetings attended by A. V. Girija Kumar?
    \item How many children does George E. Wilber. Jr. have?
    \item Who is the R\&D customer for the project  "Water on Tobacco"?
    \item What is the Box number of "University of Florida"?
    \item What is the phone number of CARR SMITH?
    \item Who is the president of CPC International Inc?
    \item Who is the senior vice president and general counsel of RJR tobacco company?
    \item Which year CLAUD T.CARNEY worked at Windsor beet lab?
    \item What the location address of NSDA?
    \item How much was the 1988 estimated expenditure committed for System buy-out- PGA Tour in the VANTAGE GOLF OPERATIONS?
    \item What is the percentage of families in Poverty in Henry county?
    \item Who is the Chairman of 'Wembley Western Australia"?
    \item Who is the author for publication "Climacteric"?
\end{itemize}

\subsection{InfoHaystack Random 20 Final Questions}

We randomly sample 20 questions in our final list of InfoHaystack as below.

\begin{itemize}

\item What was the only media for watching Team USA events live in 2008?
\item what is the total runs scored by Pietersen and Collingwood for England in 2007?
\item What was the ratio of the U.S. population to bank branches in 1970?
\item What is the number of  Flickr users worldwide as of Nov. 15, 2012?
\item How many lesbian \& bisexual women (per 1,000 population) in Canada experienced violence  in 2014?
\item How many U.S. personnels were killed during the attack at Pearl Harbor?
\item What percent of analytics jobs in India requires more than 5 years of experience according to the 2017 study?
\item what is the number of cosmetic procedures done in Japan in millions in 2011?
\item How many nonlethal gunshot wound cases were reported in America in 2009?
\item What percentage of people in the U.S use social media several times a day in 2009?
\item What was the number of employees in Hemlow in 2002?
\item How many actors acted in the series "How to make it in America"?
\item What is the number of tickets sold (in millions) in the 2012 London Olympic Games?
\item How many US households were accessing bank accounts online as per the online banking report in Jan, 2012?
\item What is the number of monthly active users of Instagram in 2016?
\item In which two years did J. G. Farrell win the Booker prize?
\item How many countries tested their first nuclear bomb after 2000?
\item How many Florida soldiers died in the Afghanistan \& Iraq war were men?
\item What percentage of people in the U.S have a social networking profile in 2010?
\item Length of what is specified for MQ-8 Fire Scout?

\end{itemize}
