# Supplementary material for: Document Haystacks: Vision-Language Reasoning Over Piles of 1000+ Documents
Source: arXiv:2411.16740 source file (2024-12-06)
Supplement: Supplementary file 2 [file eval.tex]

\section{Evaluation}
\begin{figure}[t]
    \begin{tcolorbox}[colframe=black, colback=white, coltitle=black, title=\centering\textbf{Evaluation Prompt}, sharp corners=southwest, enhanced, fonttitle=\bfseries, coltitle=white, colbacktitle=black, boxrule=0.8mm, arc=4mm]
        \begin{quote}
            \textbf{Task:} You are an evaluator. Compare the Predicted Answer with the True Answer and determine if the Predicted Answer is Correct or Incorrect.\\
            \textbf{Instructions:}
            \begin{itemize}[label=-]
                \item If the Predicted Answer provides the same information or a reasonable interpretation of the True Answer, respond with \texttt{Correct.}
                \item If the Predicted Answer does not match or does not reasonably interpret the True Answer, respond with \texttt{Incorrect.}
            \end{itemize}
            \textbf{Important:} Answer only with \texttt{Correct} or \texttt{Incorrect}—no explanations.\\
            \textbf{Input:}
            \begin{itemize}[label=-]
                \item \textbf{Question:} \{ \}
                \item \textbf{True Answer:} \{ \}
                \item \textbf{Predicted Answer:} \{ \}
            \end{itemize}
        \end{quote}
    \end{tcolorbox}
    \captionof{figure}{\textbf{The Designed Prompt for GPT Evaluation.}}
    \label{supp:eval_prompt}
\end{figure}

\textbf{GPT-based evaluation vs. traditional evaluation.} In the open visual question answering (VQA) task, the model can generate the answer in diverse format and it is hard to accurately evaluate the generated answer. 

Traditional evaluation metric such as,  \textit{Exact Match},  measures the percentage of questions where the predicted answer exactly matches one of the target answers, giving a score of zero even when the prediction is only slightly different from the correct answer.
The issue with this evaluation is that language is inherently flexible, and there can be various texts to express the same idea (\eg, ``the dog is sleeping'' vs. ``a sleeping dog'').
This flexibility often results in the \textit{Exact Match} metric failing to capture the true capability of the model sometimes. 
As shown in Fig.~\ref{supp:eval_metric1}, we show examples of zero-shot predictions from Qwen2-VL, generated without any specialized prompt design. It is clear that the \textit{Exact Match} metric fails to evaluate the accuracy of responses in this setting.
To address this, we seek a more reasonable evaluation metric that accounts for this linguistic flexibility.
With the recent advancements in LLMs, GPT-based evaluations are growing in popularity. due to their closer alignment with human behavior in interpreting language.
We carefully design an evaluation prompt for GPT to score the predicted answer against the true answer. The evaluation prompt is structured in Fig~\ref{supp:eval_prompt}.

\begin{figure}[t]
	\begin{center}
        \includegraphics[width=1.0\linewidth]{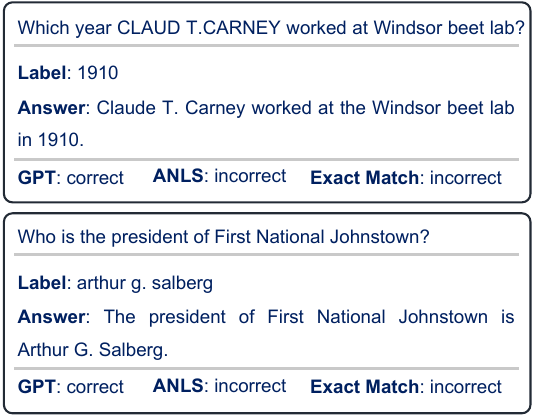}
	\end{center}
	\captionsetup{font=small}
        \vspace{-3mm}
        \caption{\textbf{Zero-Shot VQA without using Task-Specific Prompt.} Without limiting the output space, traditional metrics cannot evaluate model performance even when the model's answer is correct.}
	\label{supp:eval_metric1}
\end{figure}

\begin{figure}[t]
	\begin{center}
        \includegraphics[width=1.0\linewidth]{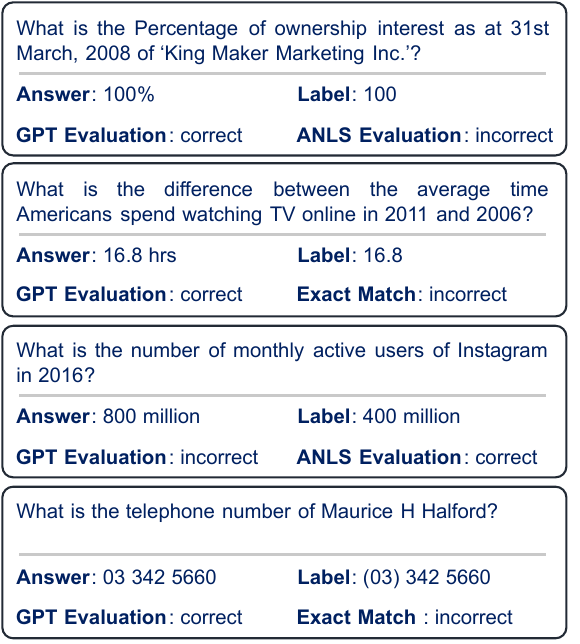}
	\end{center}
	\captionsetup{font=small}
        \vspace{-3mm}
        \caption{\textbf{Zero-Shot VQA with using Task-Specific Prompt.} Even when the output space is limited, traditional metrics sometimes fail to evaluate model performance correctly, even if the model's answer is correct.}
	\label{supp:eval_metric2}
\end{figure}

We validate the consistency of the proposed GPT-based evaluation with human judgments, aiming to demonstrate its effectiveness compared to traditional metrics, \ie, \textit{Exact Match} and \textit{ANLS}. Note that for \textit{ANLS}, we consider a similarity score greater than 0.8 as correct.
As illustrated in Fig.~~\ref{supp:eval_metric2}, traditional metrics can sometimes misjudge zero-shot prediction. This limitation becomes evident in scenarios where the flexibility of responses is crucial.
%
% While task-specific prompts can guide models to provide more constrained outputs, they are often impractical in real-world applications as it is difficult for us to know the distribution of answers beforehand.
%∂
Note that we explicitly ask the model to ``Answer the question using a single word or phrase.''~\footnote{\url{https://github.com/EvolvingLMMs-Lab/lmms-eval}} This prompt ensures brevity and facilitates a fair comparison between predicted and target answers. 

We report the performance of different evaluation metrics on DocHaystack-100 and InforHaystack-100 in Tab.~\ref{tab:eval_metrics}. The results show that the introduced GPT-based metric aligns closely with human evaluation, outperforming traditional metrics.
Based on these experimental results, we choose GPT-based evaluation for better accuracy.

\begin{table}[h]
\centering
\resizebox{1.0 \linewidth}{!}{
    \begin{tabular}{c ccc}
    \toprule
    Evaluation Metric& DocHaystack 100& InfoHaystack 100\\
    % \midrule
    \cmidrule(r){1-1} \cmidrule(lr){2-2} \cmidrule(lr){3-3}
    Human & 78.90 & 62.58 \\
    Exact Match & 69.72 & 58.71 \\
    ANLS & 73.39 & 60.65 \\
    \rowcolor{TealBlue}
    GPT & 78.90 & 62.58 \\
    \bottomrule
    \end{tabular}
}
\caption{\textbf{Accuracy of Qwen2-VL on DocHaystack-100 and InfoHaystack-100.} We report different accuracy using different evaluation metrics.}
\label{tab:eval_metrics}
\end{table}
