# Supplementary material for: Document Haystacks: Vision-Language Reasoning Over Piles of 1000+ Documents
Source: arXiv:2411.16740 source file (2024-12-06)
Supplement: Supplementary file 4 [file retrieval.tex]

\section{Image Retrieval}

We select retrieved images based on their similarity to the question and present the three most relevant images retrieved using different methods (\ie, V-RAG-based retrieval, CLIP-based retrieval, SigLIP-based retrieval, OpenCLIP-based Retrieval): Fig.~\ref{supp:retrieval1}~--~\ref{supp:retrieval3} for DocHaystack and Fig.~\ref{supp:retrieval4}~--~\ref{supp:retrieval6} for InfoHaystack.
In these figures, the red box outside the retrieved image highlights the ground truth image paired with the question. The red box within each retrieved image shows the related information to the question. The yellow box in the ground truth image paired with the question shows the ground truth answer for the question. As can be seen in these figures, our proposed V-RAG performs well in question-related image retrieval.

\begin{figure*}[t!]
	\begin{center}
        \includegraphics[width=\linewidth]{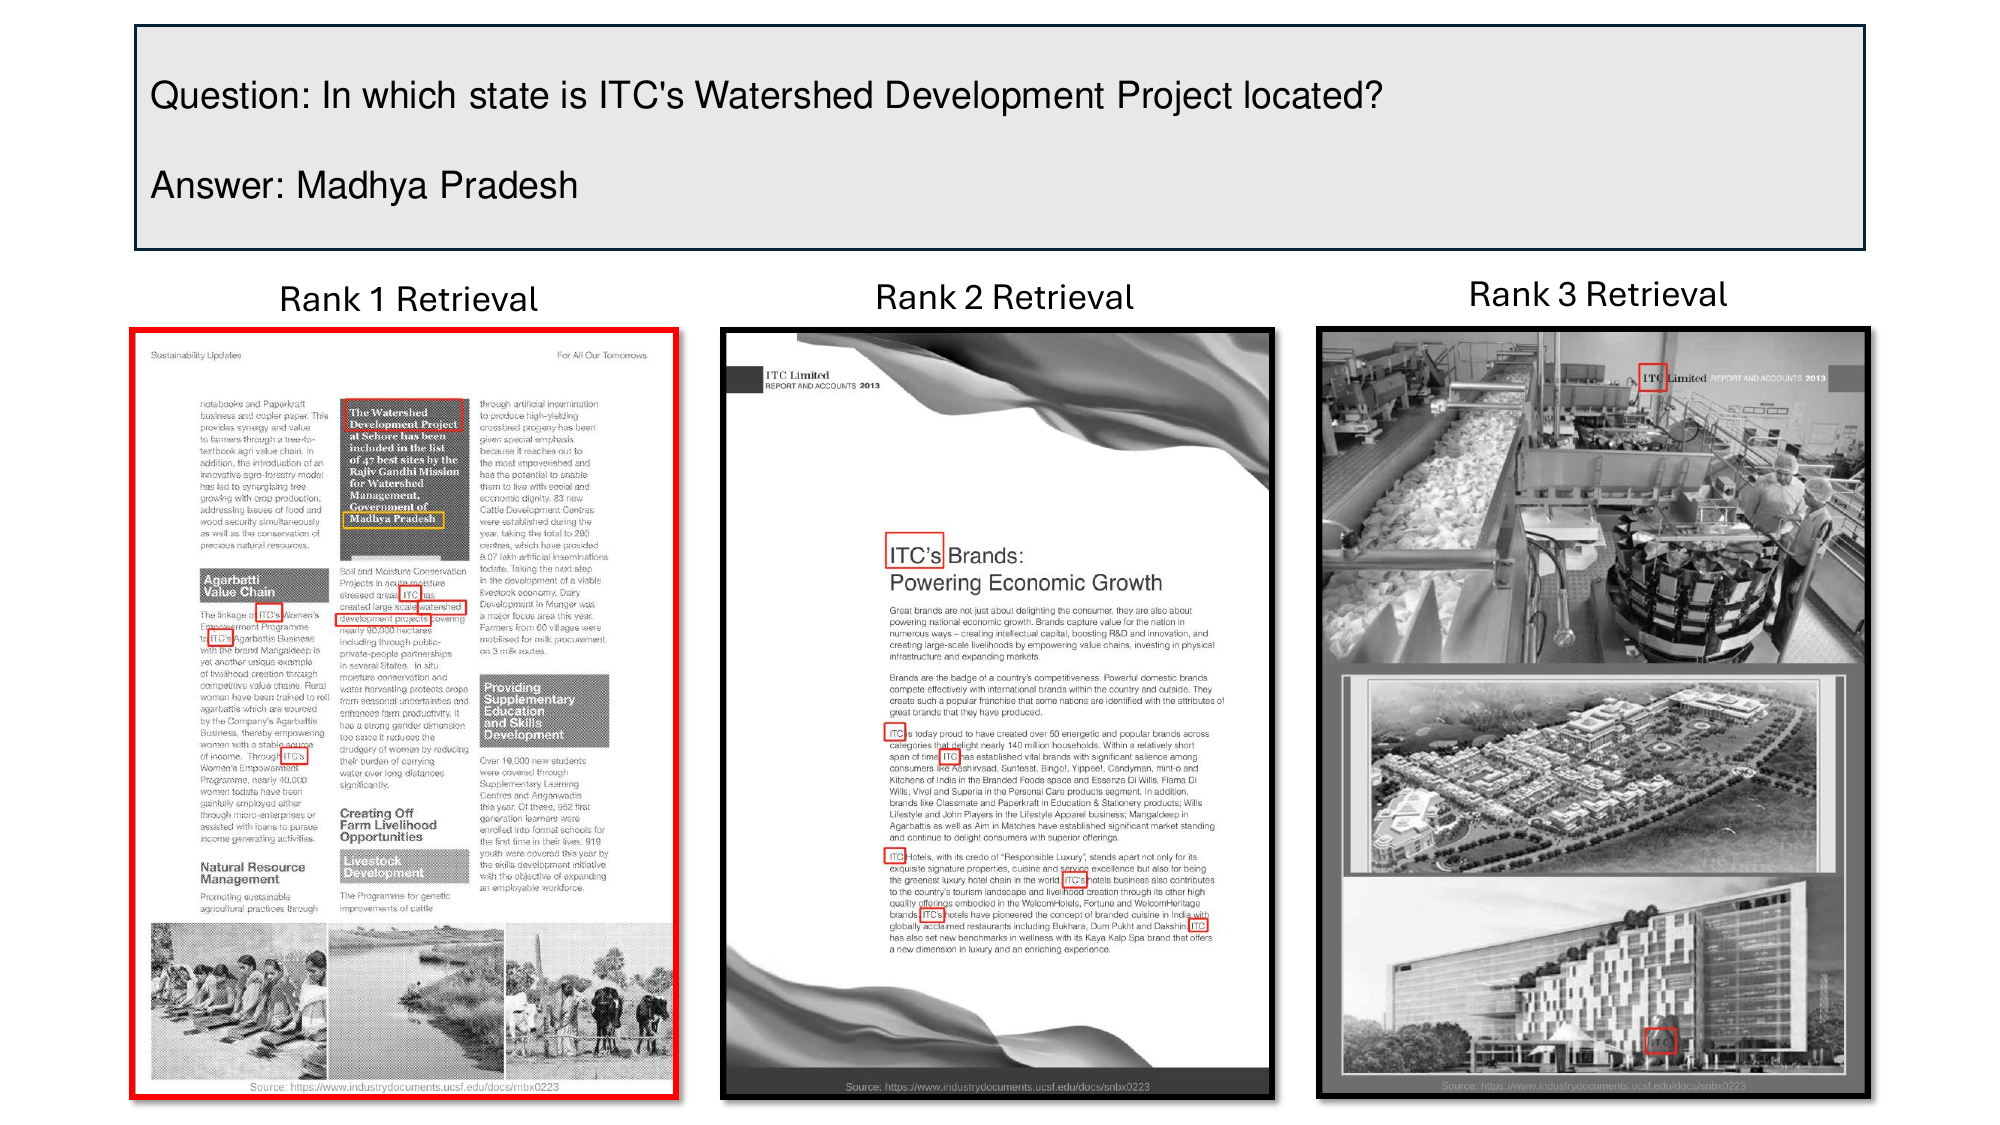}
	\end{center}
	\captionsetup{font=small}
	\caption{The three images most similar to the question retrieved using V-RAG in DocHaystack. The red box highlights the ground truth image paired with the question.
    % The red circle in each image shows the related information to the question. The yellow circle in the ground truth image paired with the question shows the ground twruth answer for the question.
    }
	\label{supp:retrieval1}
    \vspace{-0.3cm}
\end{figure*}

\begin{figure*}[t!]
	\begin{center}
        \includegraphics[width=\linewidth]{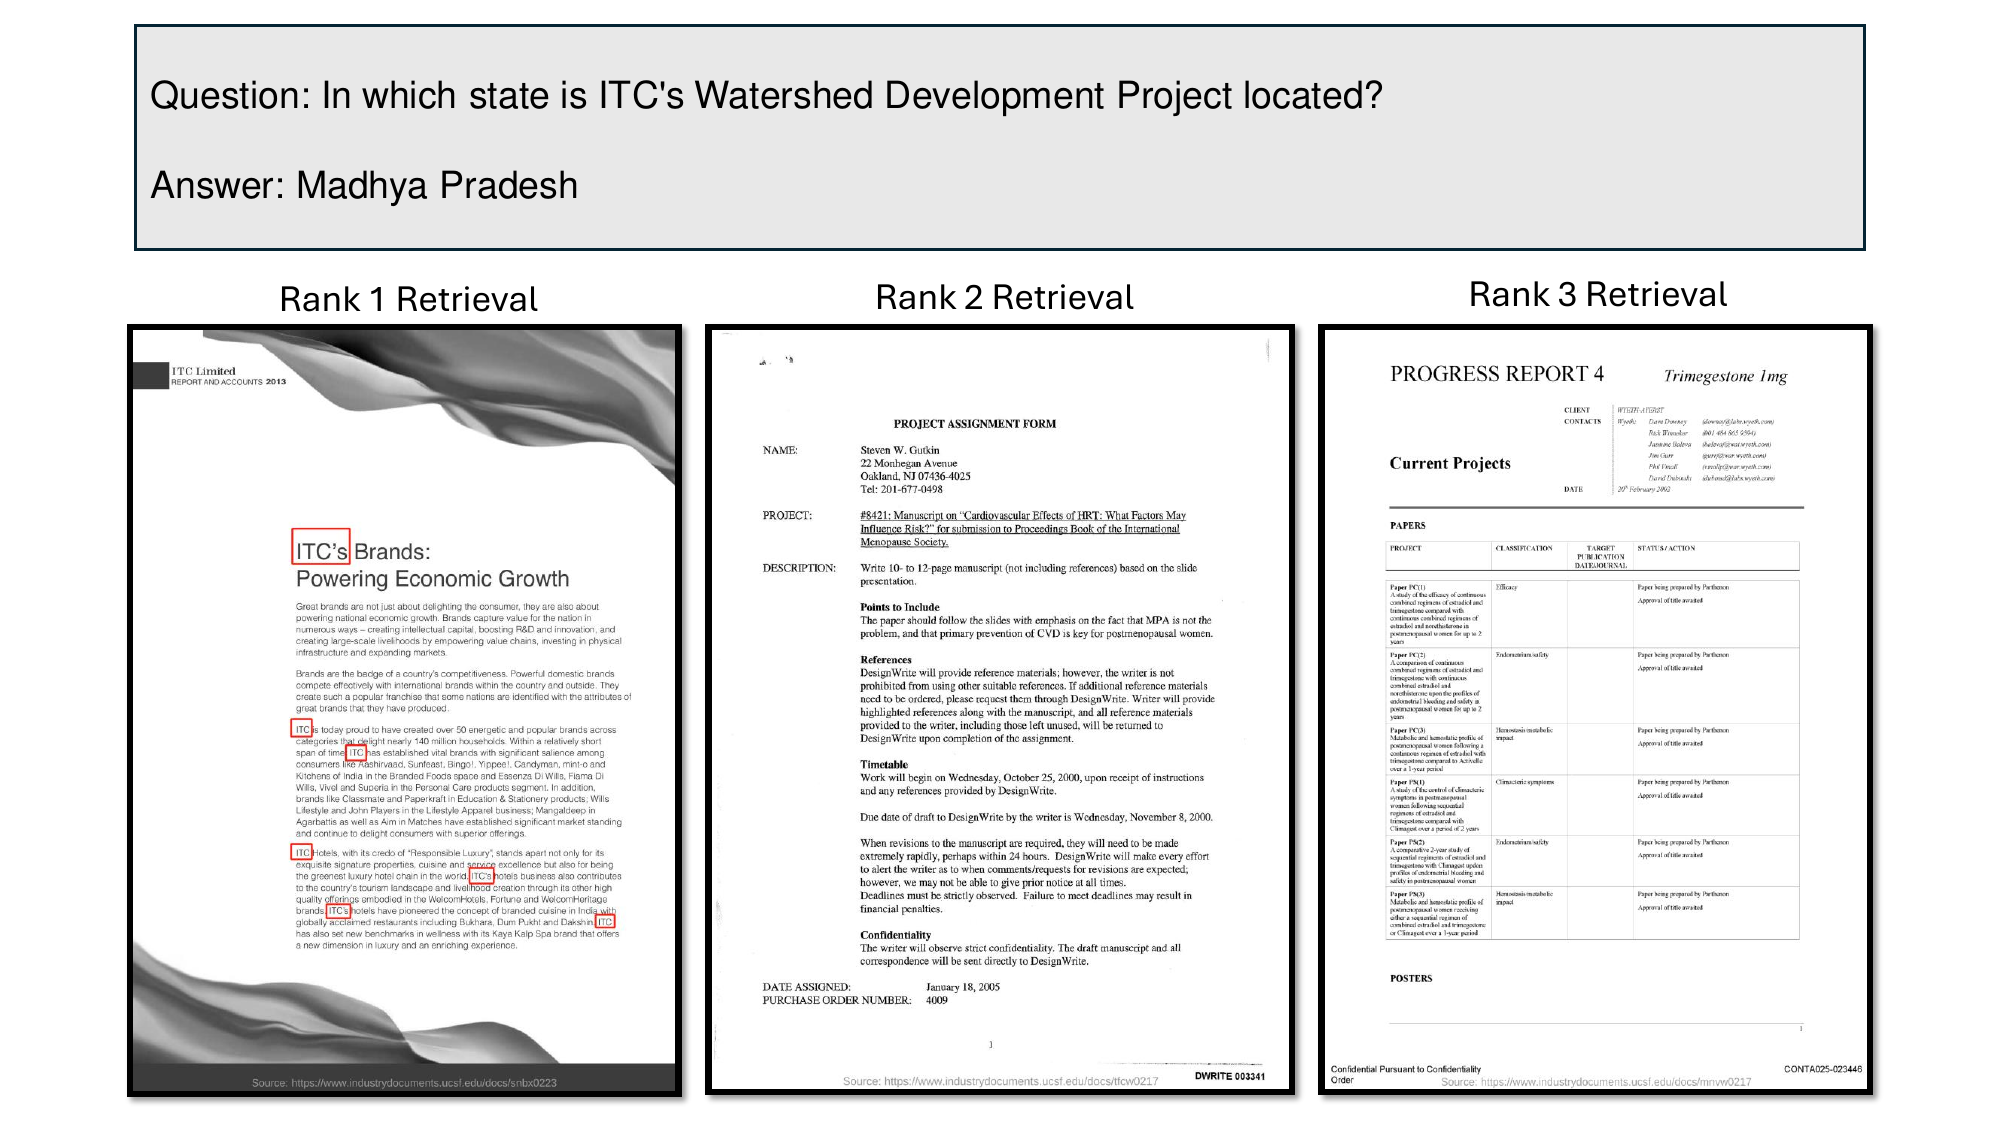}
	\end{center}
	\captionsetup{font=small}
	\caption{The three images most similar to the question retrieved using CLIP in DocHaystack. The red box highlights the ground truth image paired with the question.
    % The red circle in each image shows the related information to the question. The yellow circle in the ground truth image paired with the question shows the ground truth answer for the question.
    }
	\label{supp:retrieval2}
    \vspace{-0.3cm}
\end{figure*}

\begin{figure*}[t!]
	\begin{center}
        \includegraphics[width=\linewidth]{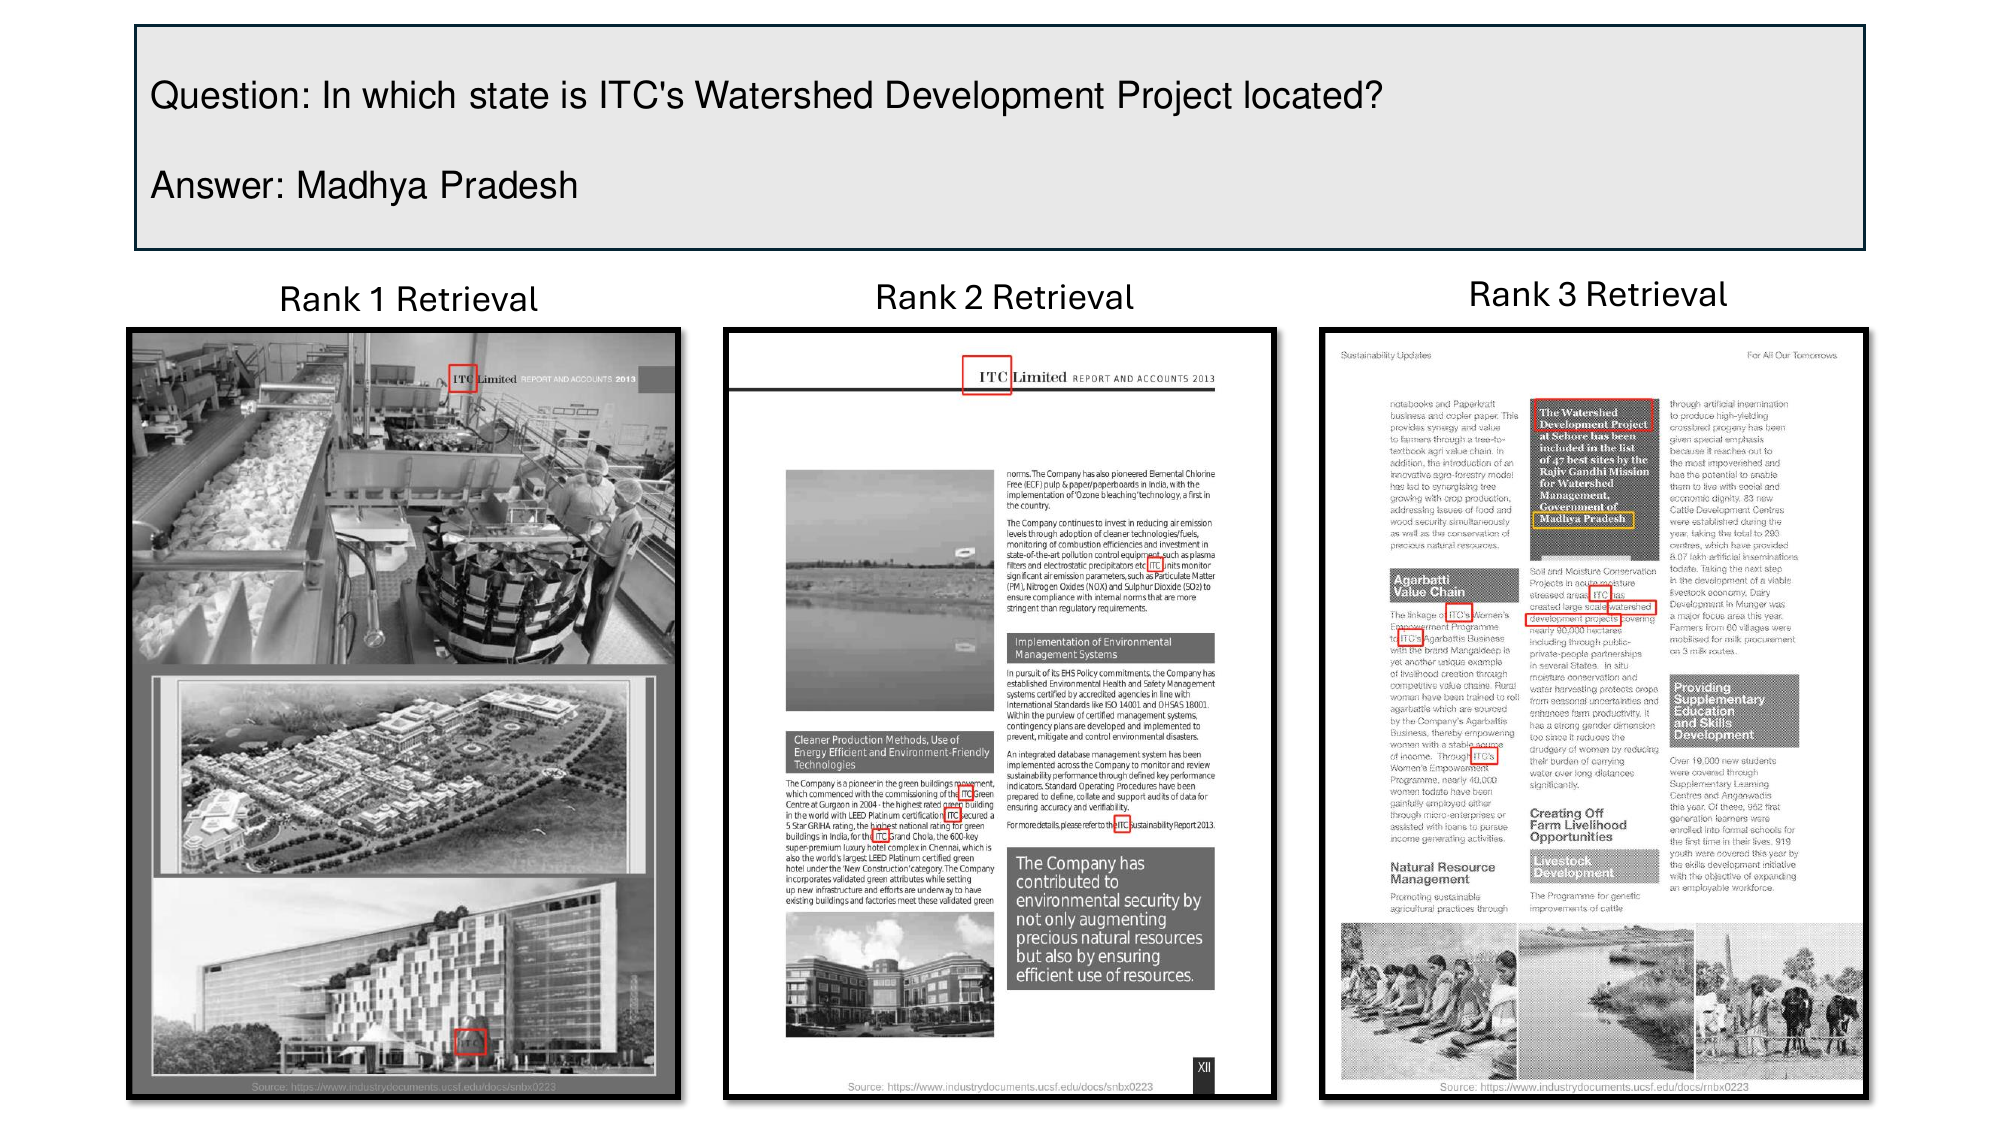}
	\end{center}
	\captionsetup{font=small}
	\caption{The three images most similar to the question retrieved using SigLIP in DocHaystack. The red box highlights the ground truth image paired with the question.
    % The red circle in each image shows the related information to the question. The yellow circle in the ground truth image paired with the question shows the ground truth answer for the question.
    }
	\label{supp:retrieval3}
    \vspace{-0.3cm}
\end{figure*}

\begin{figure*}[t!]
	\begin{center}
        \includegraphics[width=\linewidth]{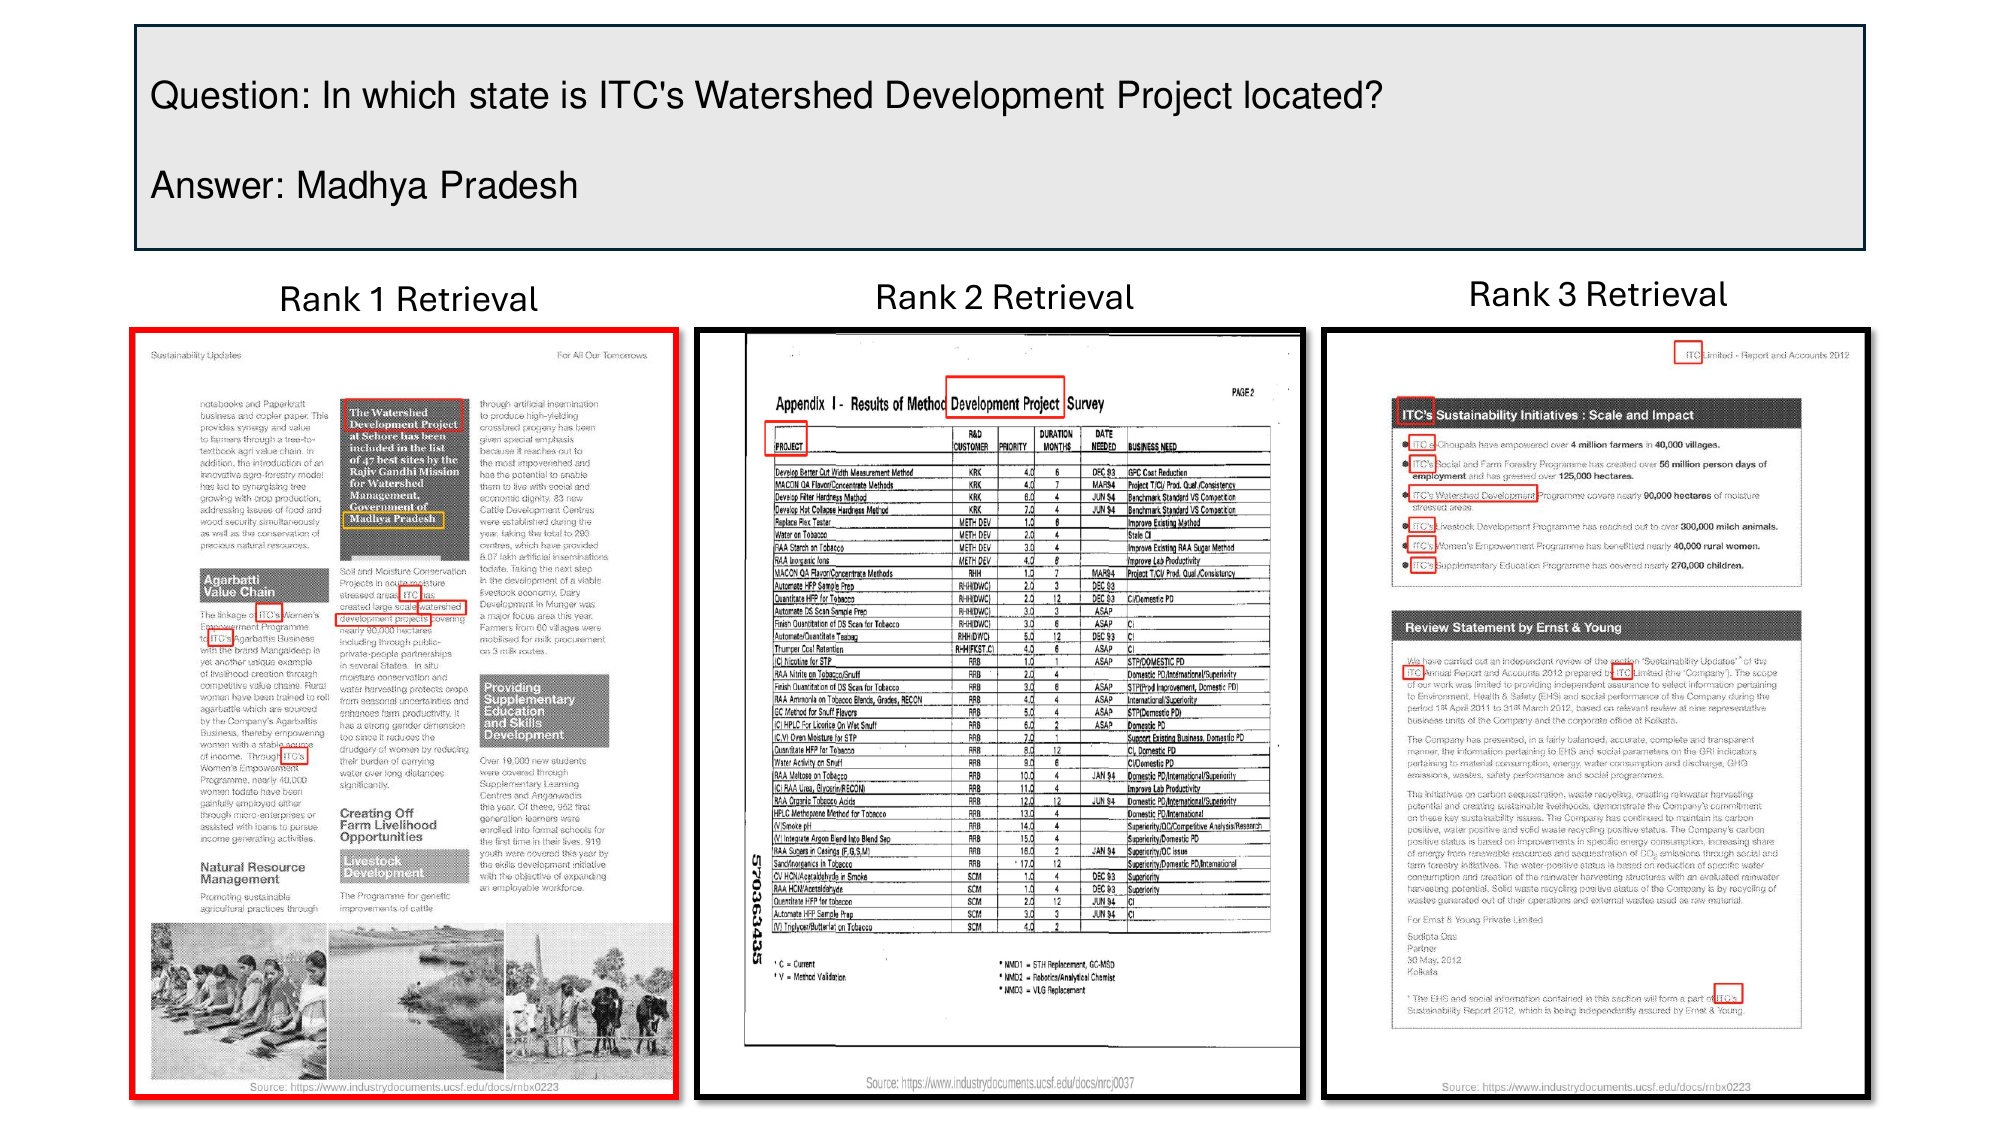}
	\end{center}
	\captionsetup{font=small}
	\caption{The three images most similar to the question retrieved using OpenCLIP in DocHaystack. The red box highlights the ground truth image paired with the question.
    % The red circle in each image shows the related information to the question. The yellow circle in the ground truth image paired with the question shows the ground truth answer for the question.
    }
	\label{supp:retrieval4}
    \vspace{-0.3cm}
\end{figure*}

\begin{figure*}[t!]
	\begin{center}
        \includegraphics[width=\linewidth]{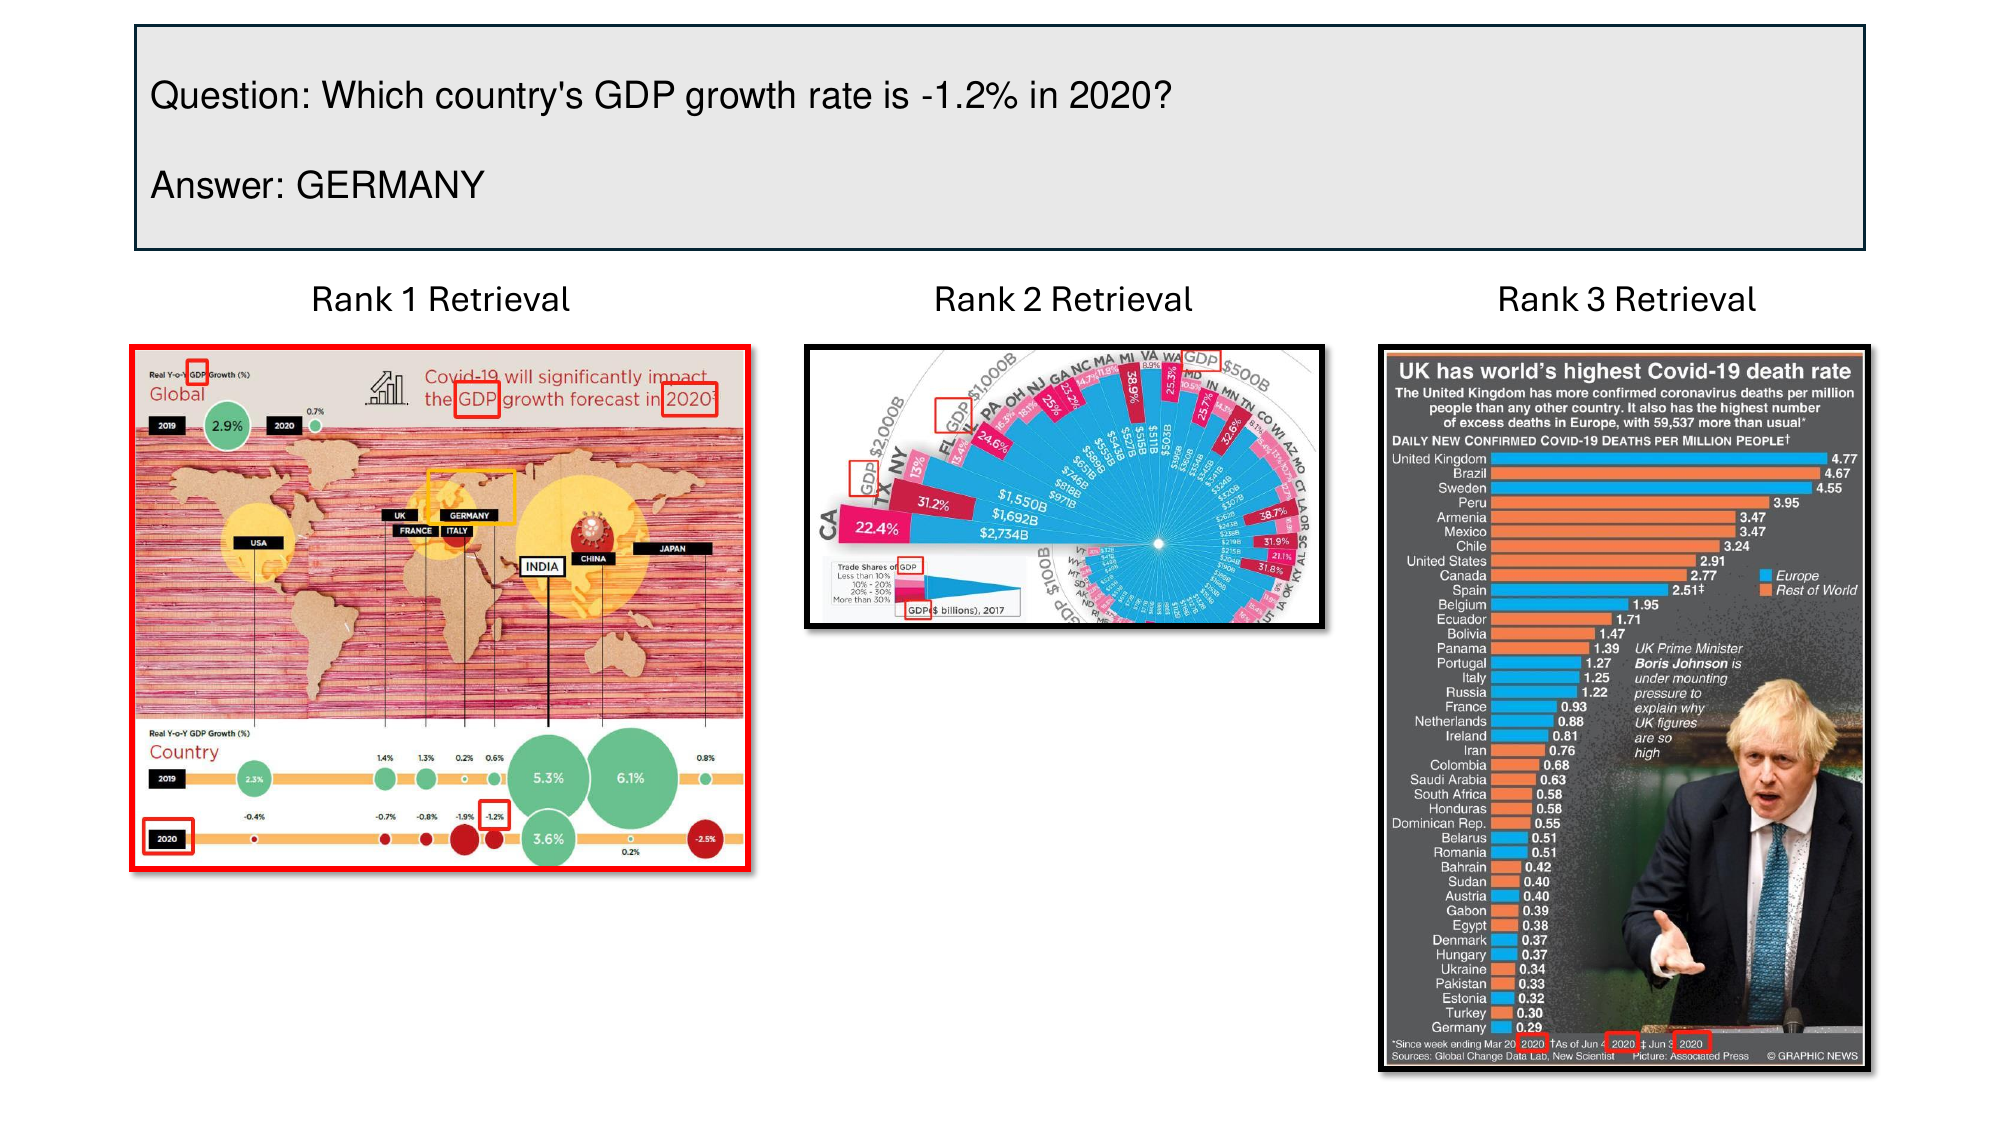}
	\end{center}
	\captionsetup{font=small}
	\caption{The three images most similar to the question retrieved using V-RAG in InfoHaystack. The red box highlights the ground truth image paired with the question.
    % The red circle in each image shows the related information to the question. The yellow circle in the ground truth image paired with the question shows the ground truth answer for the question.
    }
	\label{supp:retrieval5}
    \vspace{-0.3cm}
\end{figure*}

\begin{figure*}[t!]
	\begin{center}
        \includegraphics[width=\linewidth]{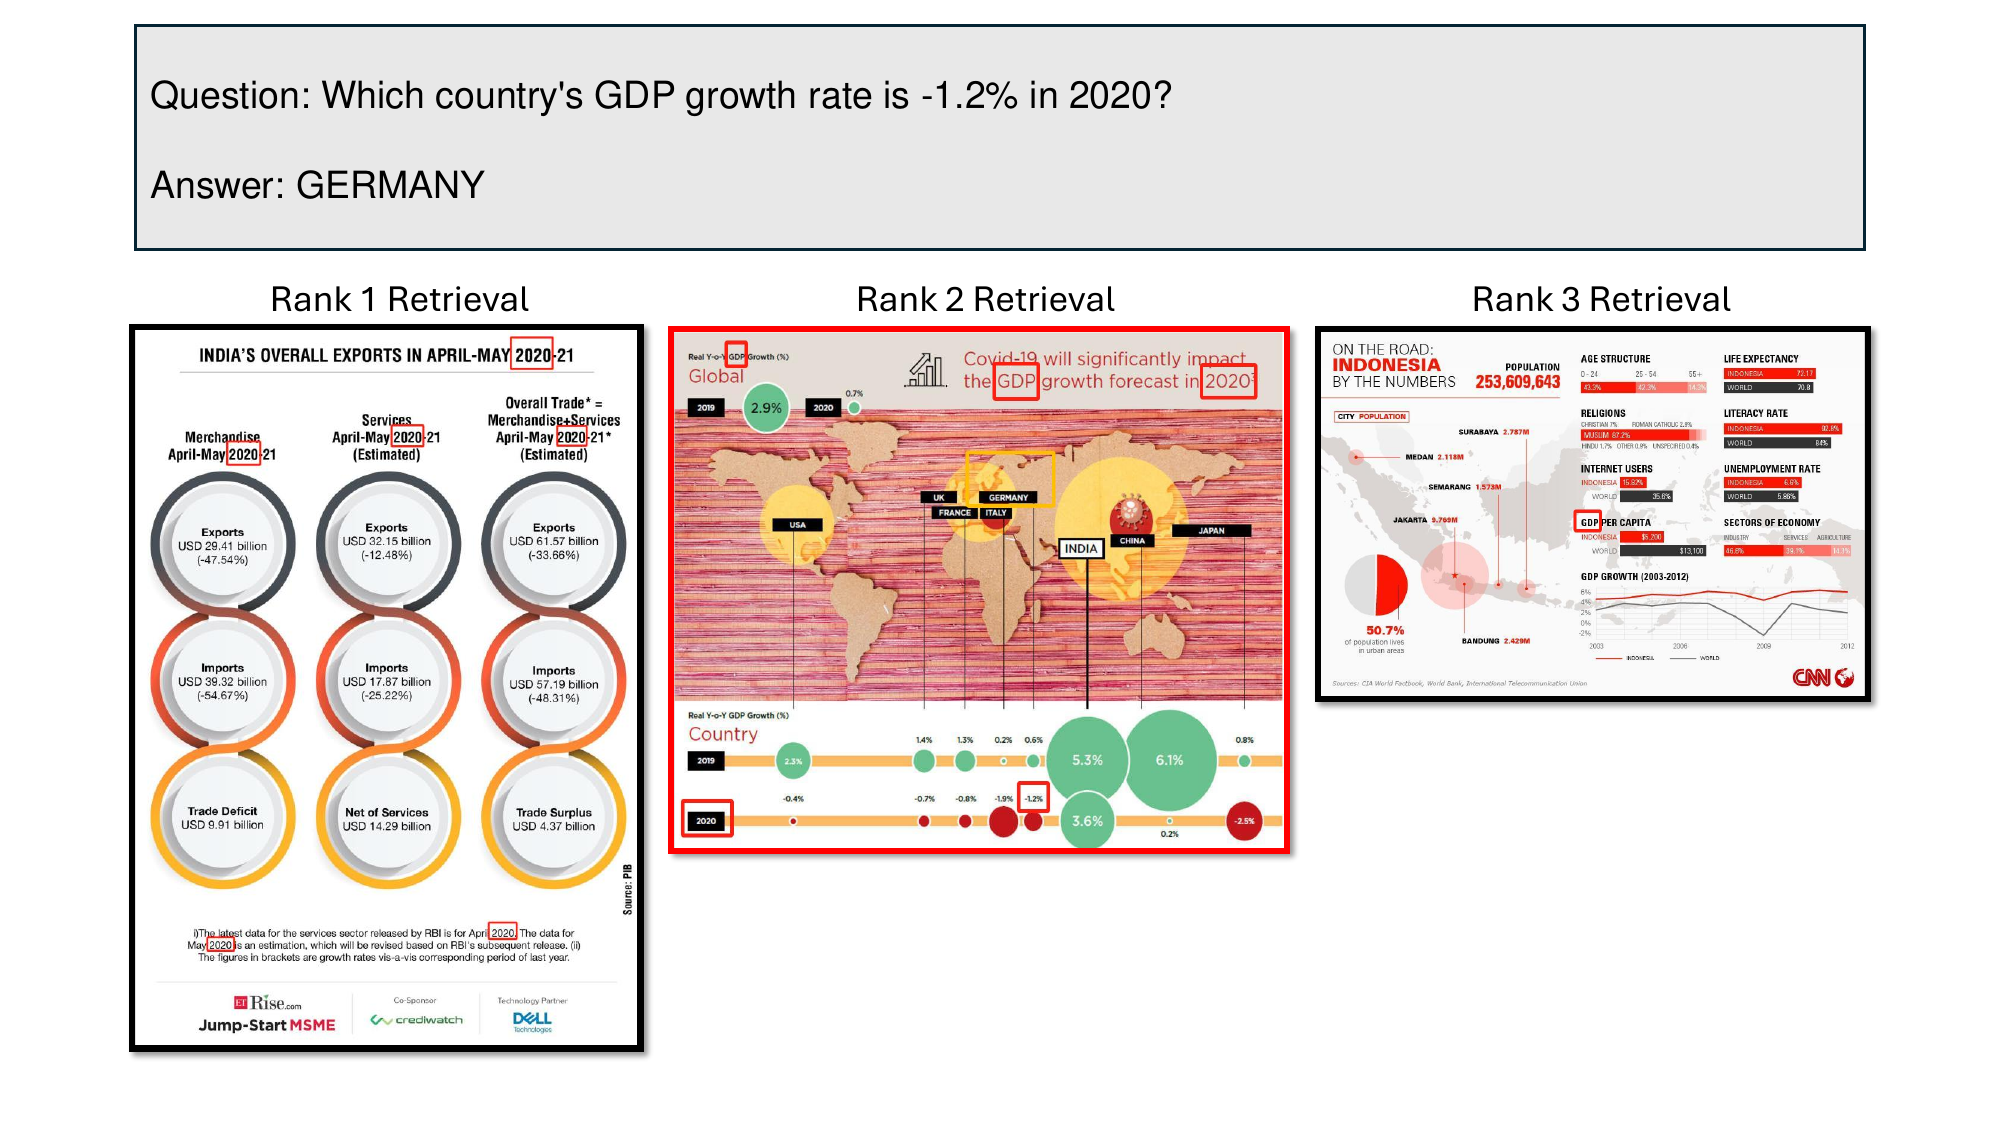}
	\end{center}
	\captionsetup{font=small}
	\caption{The three images most similar to the question retrieved using CLIP in InfoHaystack. The red box highlights the ground truth image paired with the question.
    % The red circle in each image shows the related information to the question. The yellow circle in the ground truth image paired with the question shows the ground truth answer for the question.
    }
	\label{supp:retrieval6}
    \vspace{-0.3cm}
\end{figure*}

\begin{figure*}[t!]
	\begin{center}
        \includegraphics[width=\linewidth]{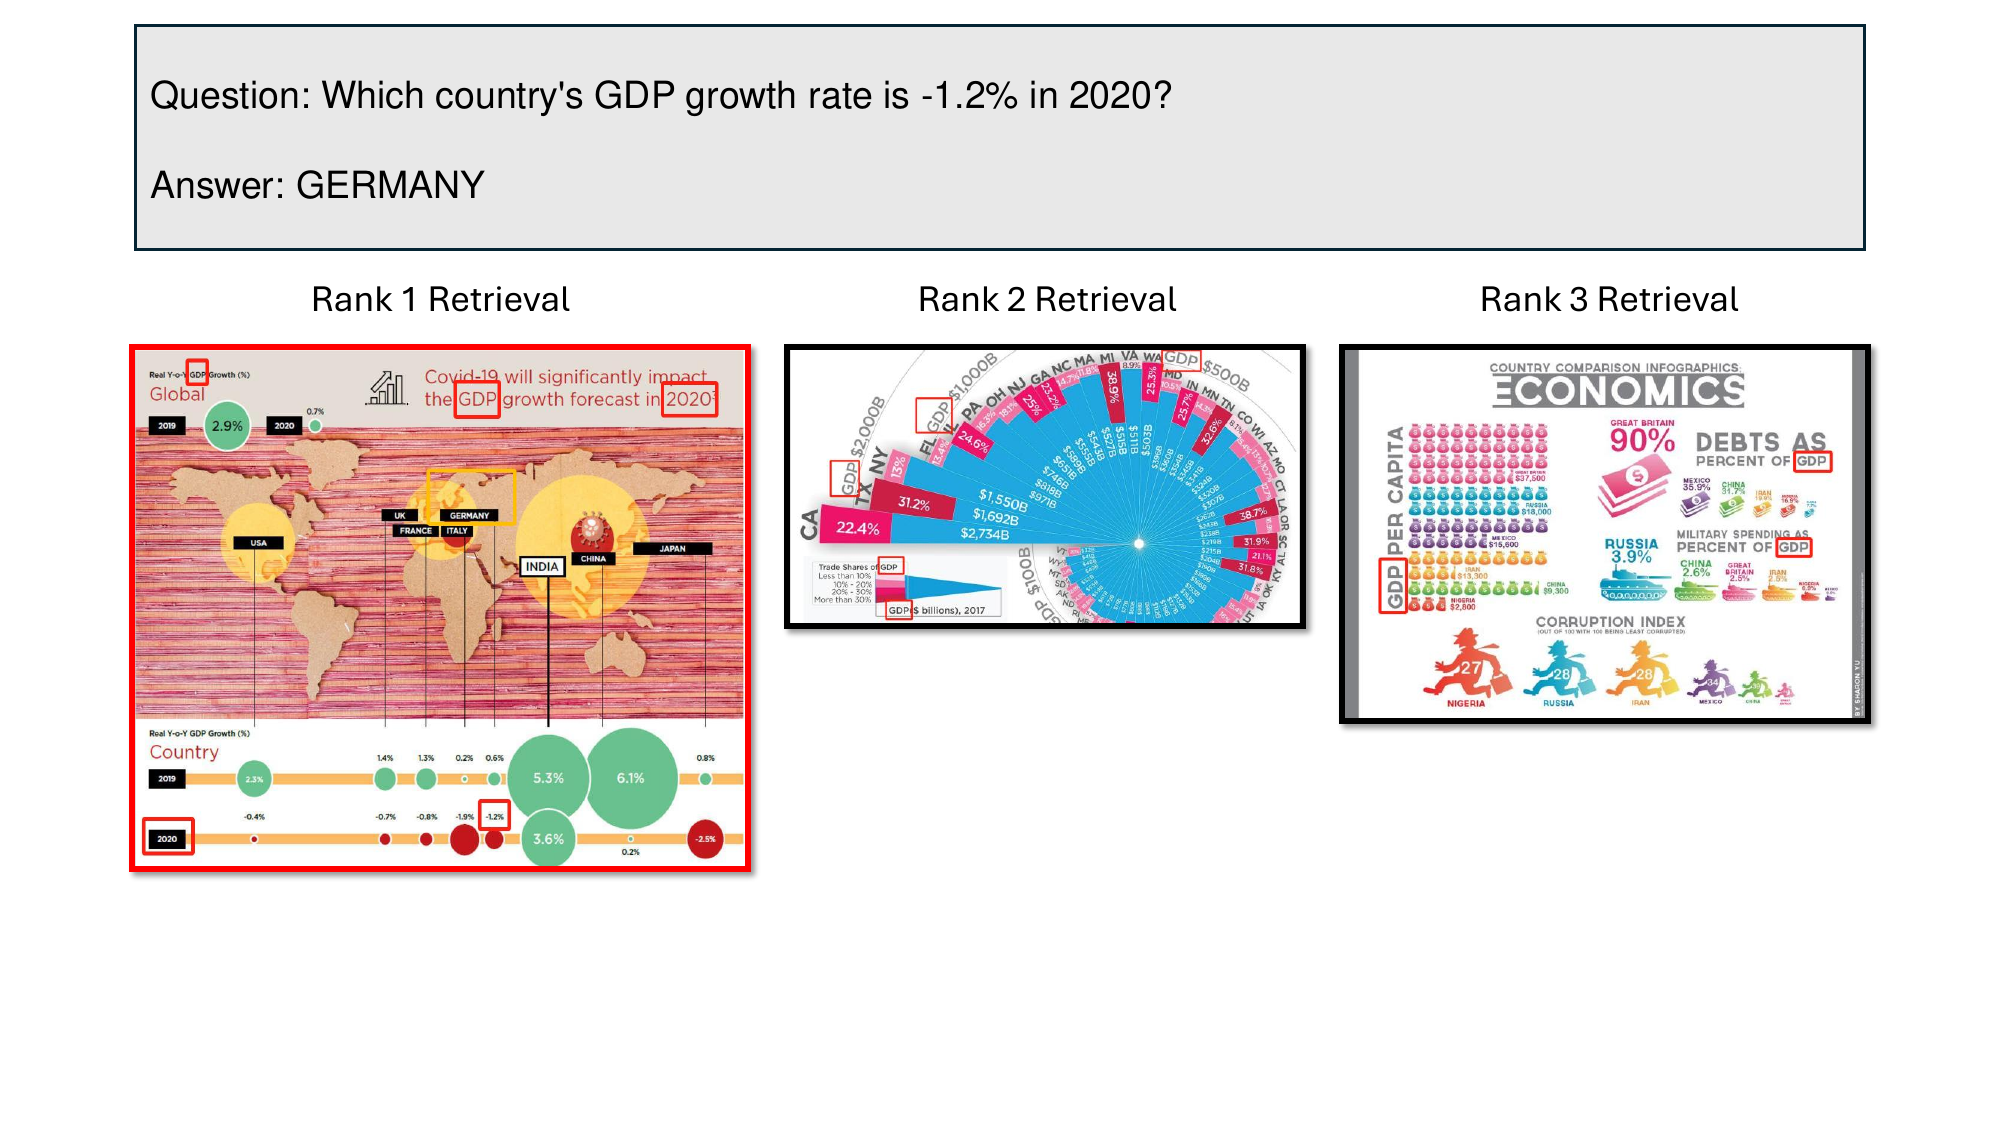}
	\end{center}
	\captionsetup{font=small}
	\caption{The three images most similar to the question retrieved using SigLIP in InfoHaystack. The red box highlights the ground truth image paired with the question.
    % The red circle in each image shows the related information to the question. The yellow circle in the ground truth image paired with the question shows the ground truth answer for the question.
    }
	\label{Rank_SIGLIP_Info}
    \vspace{-0.3cm}
\end{figure*}

\begin{figure*}[t!]
	\begin{center}
        \includegraphics[width=\linewidth]{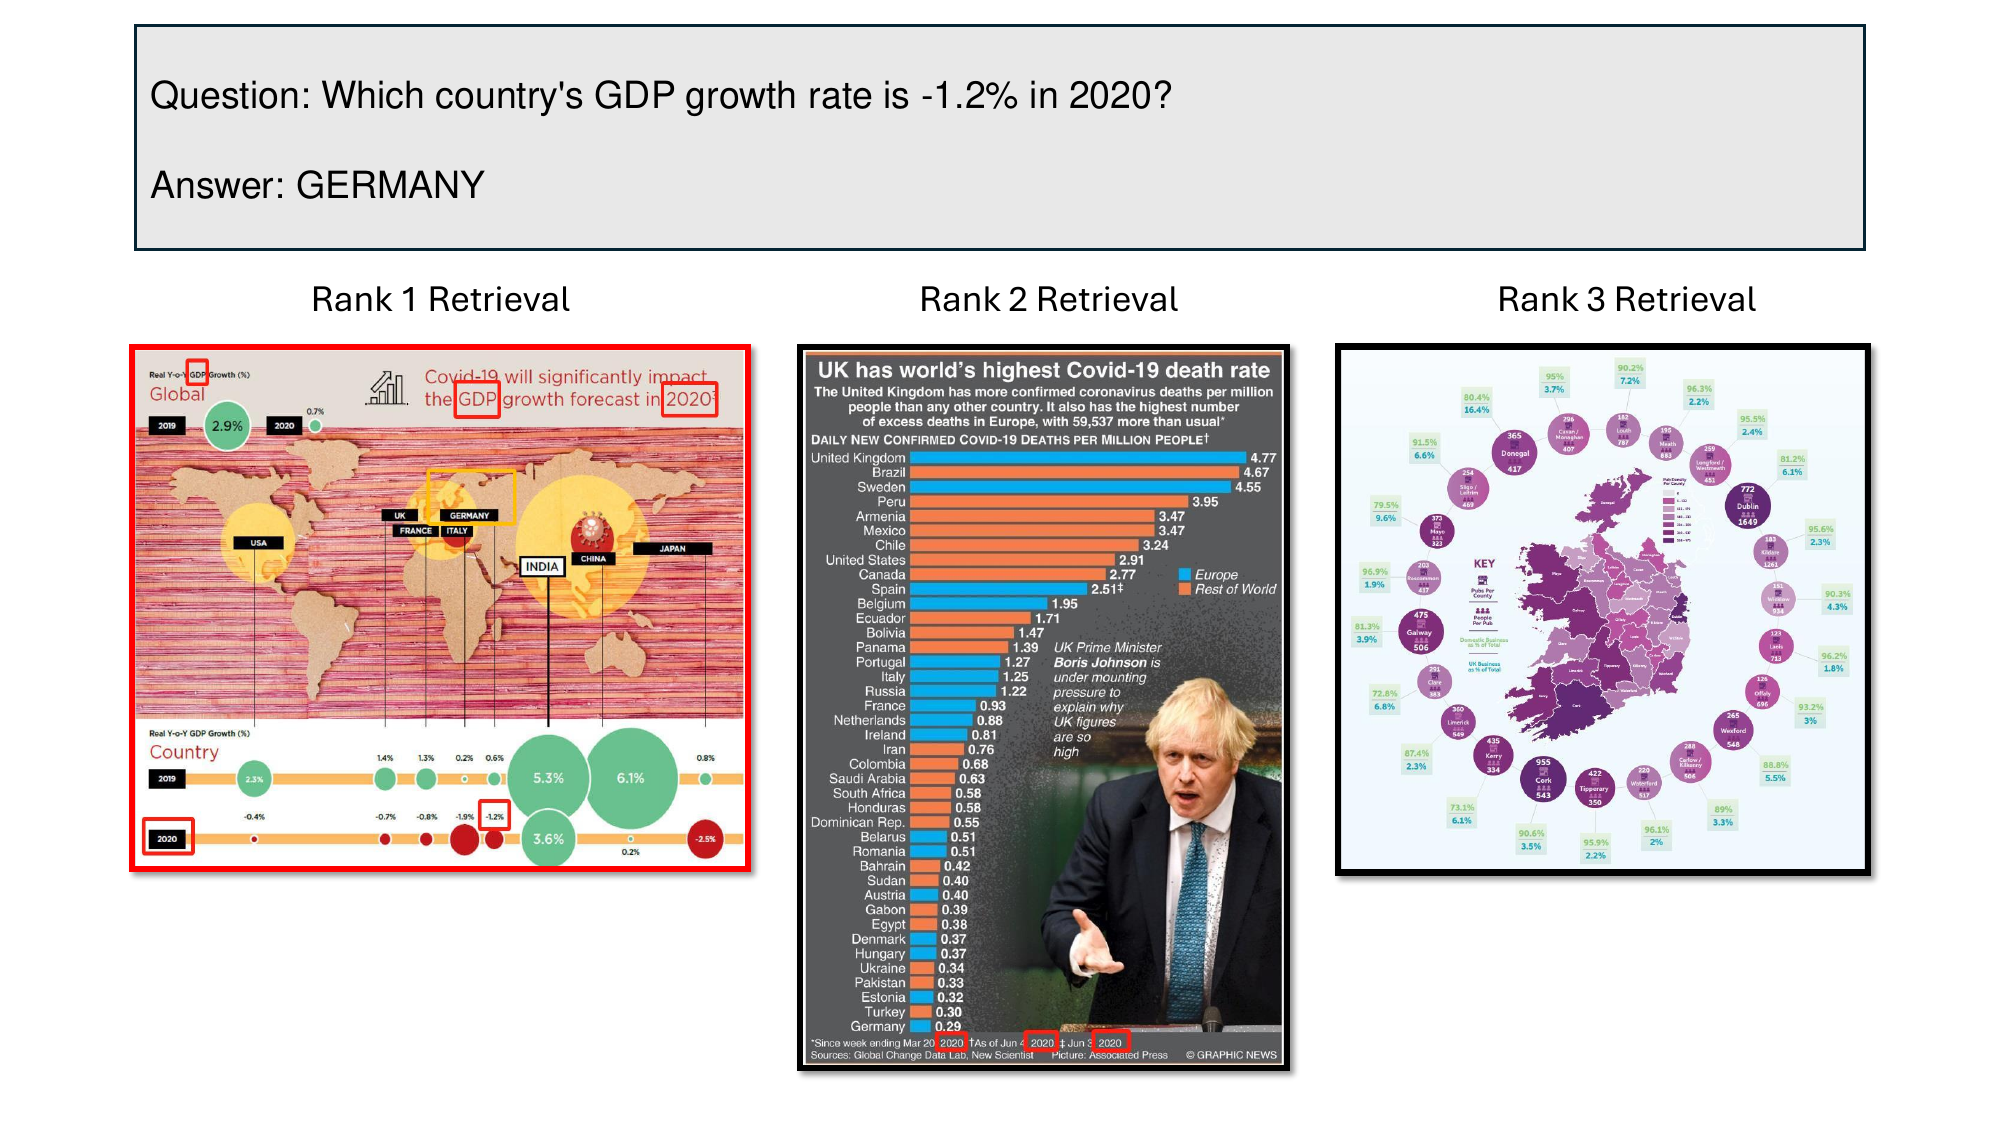}
	\end{center}
	\captionsetup{font=small}
	\caption{The three images most similar to the question retrieved using OpenCLIP in DocHaystack. The red box highlights the ground truth image paired with the question.
    % The red circle in each image shows the related information to the question. The yellow circle in the ground truth image paired with the question shows the ground truth answer for the question.
    }
	\label{Rank_OpenCLIP_Info}
    \vspace{-0.3cm}
\end{figure*}

% \section{General-Question LLM Filtering}
% \subsection{DocHaystack}
