# Supplementary material for: Document Haystacks: Vision-Language Reasoning Over Piles of 1000+ Documents
Source: arXiv:2411.16740 source file (2024-12-06)
Supplement: Supplementary file 5 [file supplementary.tex]

% % CVPR 2025 Paper Template; see https://github.com/cvpr-org/author-kit

% \documentclass[10pt,twocolumn,letterpaper]{article}

% %%%%%%%%% PAPER TYPE  - PLEASE UPDATE FOR FINAL VERSION
% % \usepackage{cvpr}              % To produce the CAMERA-READY version
% \usepackage[review]{cvpr}      % To produce the REVIEW version
% % \usepackage[pagenumbers]{cvpr} % To force page numbers, e.g. for an arXiv version

% % customize package
% \usepackage{multirow}
% \usepackage{color, colortbl}
% \definecolor{Gray1}{gray}{0.9}
% \definecolor{Gray2}{gray}{1.0}
% % \definecolor{TealBlue}{gray}{0.9}
% \usepackage{booktabs}

% % \definecolor{TealBlue}{rgb}{0.61, 0.87, 1.0}
% \definecolor{TealBlue}{rgb}{1.0, 0.97, 0.91}

% \newcommand{\junjie}[1]{\textcolor[rgb]{1.0, 0.714, 0.757}{\textbf{Junjie:} #1}}
% \usepackage{pifont}
% % \newcommand{\x}[1]{\textcolor[rgb]{1.0, 0.714, 0.757}{\ding{53}}}
% \newcommand{\x}[0]{\ding{53}}

% \usepackage{colortbl} % Add this line to your preamble to use colors
% % \usepackage{hyperref}

% \usepackage{placeins}


% % Import additional packages in the preamble file, before hyperref
% \input{preamble}

% % It is strongly recommended to use hyperref, especially for the review version.
% % hyperref with option pagebackref eases the reviewers' job.
% % Please disable hyperref *only* if you encounter grave issues, 
% % e.g. with the file validation for the camera-ready version.
% %
% % If you comment hyperref and then uncomment it, you should delete *.aux before re-running LaTeX.
% % (Or just hit 'q' on the first LaTeX run, let it finish, and you should be clear).
% \definecolor{cvprblue}{rgb}{0.21,0.49,0.74}


% \definecolor{firebrick}{rgb}{0.7, 0.13, 0.13}
% \definecolor{darkpastelgreen}{rgb}{0.01, 0.75, 0.24}
% \definecolor{deepskyblue}{rgb}{0.0, 0.75, 1.0}
% \definecolor{mypink2}{rgb}{.99,.96,.98}%浅
% \definecolor{mypink1}{rgb}{.99,.93,.98}
% \definecolor{mypink}{rgb}{.99,.90,.98}%深
% % \definecolor{mypink}{rgb}{.99,.91,.95}
% \definecolor{mygray}{rgb}{.95,.95,.95}
% \definecolor{lv14}{rgb}{0.5,0.5,0.5}

% \renewcommand{\thesection}{\Alph{section}}
% \usepackage[most]{tcolorbox} 

% \usepackage[pagebackref,breaklinks,colorlinks,allcolors=cvprblue]{hyperref}

% %%%%%%%%% PAPER ID  - PLEASE UPDATE
% \def\paperID{8243} % *** Enter the Paper ID here
% \def\confName{CVPR}
% \def\confYear{2025}

% %%%%%%%%% TITLE - PLEASE UPDATE
% % \title{Document Haystack Benchmarks: Ask Any Visual Questions over 1K Documents}

% % \title{Document Haystack Benchmarks: Ask over 1K Documents}

% %\title{Document Haystack Benchmarks: VQA over 1K Documents}
% \title{Appendix for Document Haystacks:  Vision-Language Reasoning Over Piles of \\1000+ Documents}

% %%%%%%%%% AUTHORS - PLEASE UPDATE
% \author{First Author\\
% Institution1\\
% Institution1 address\\
% {\tt\small firstauthor@i1.org}
% % For a paper whose authors are all at the same institution,
% % omit the following lines up until the closing ``}''.
% % Additional authors and addresses can be added with ``\and'',
% % just like the second author.
% % To save space, use either the email address or home page, not both
% \and
% Second Author\\
% Institution2\\
% First line of institution2 address\\
% {\tt\small secondauthor@i2.org}
% }

% \begin{document}

% \maketitlesupplementary

% \input{supp/eval}
% \input{supp/retrieval}
% \clearpage
% \input{supp/question}



% % {
% %     \small
% %     \bibliographystyle{ieeenat_fullname}
% %     \bibliography{main}
% % }

% % WARNING: do not forget to delete the supplementary pages from your submission 
% % \input{sec/X_suppl}



% \end{document}
% \end{document}
